# Supplementary material for: RobotPerf: An Open-Source, Vendor-Agnostic, Benchmarking Suite for Evaluating Robotics Computing System Performance
Source: arXiv:2309.09212 source file (2024-01-29)
Supplement: Supplementary file 1 [file 9_appendix.tex]

%%%%%%%%%%%%%%%%%%%%%%%%%%%%%%%%%%%%%%%%%%%%%%%%%%%%%%%%

%\subsection*{Robotic Perception Benchmarks}
\label{sec:appendix_perception}

\begin{figure*}[tbp]
\centering

% a1
\begin{subfigure}[t]{0.32\textwidth}  
\centering
\raisebox{-\height}{\includegraphics[width=\textwidth]{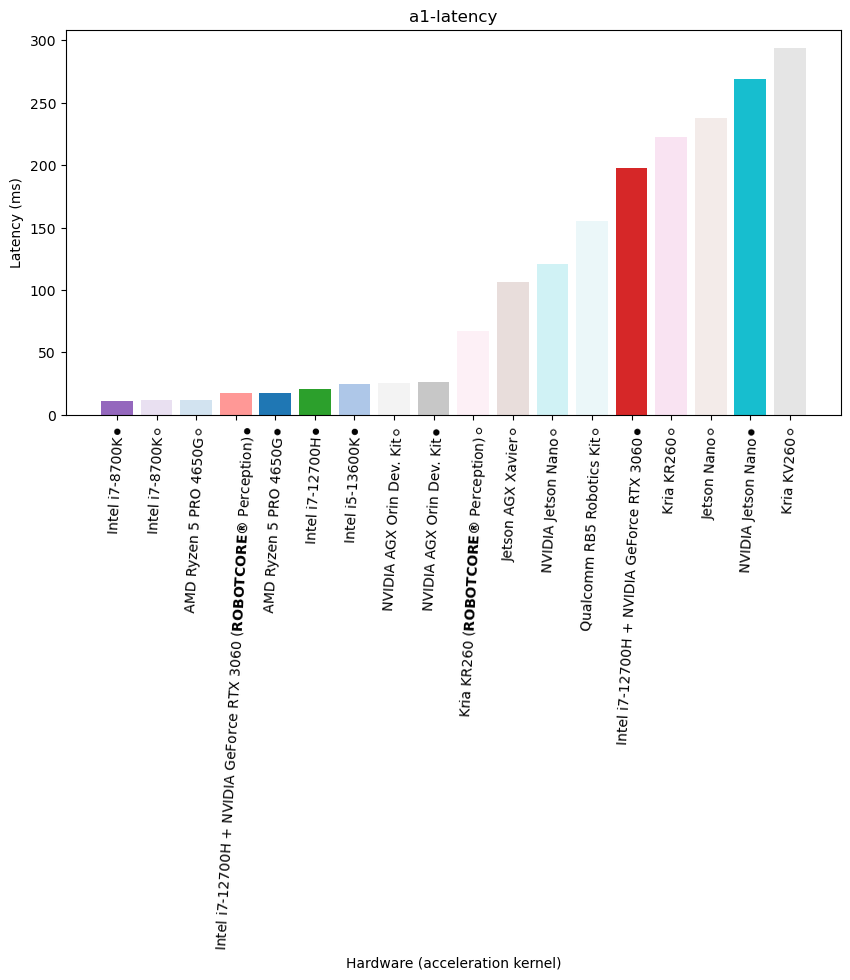}}
\caption{Best latency results for \texttt{a1} benchmark.}
\label{subfig:besta1latency}
\end{subfigure}
\hfill % ensures that they are side by side
\begin{subfigure}[t]{0.32\textwidth}
\centering
\raisebox{-\height}{\includegraphics[width=\textwidth]{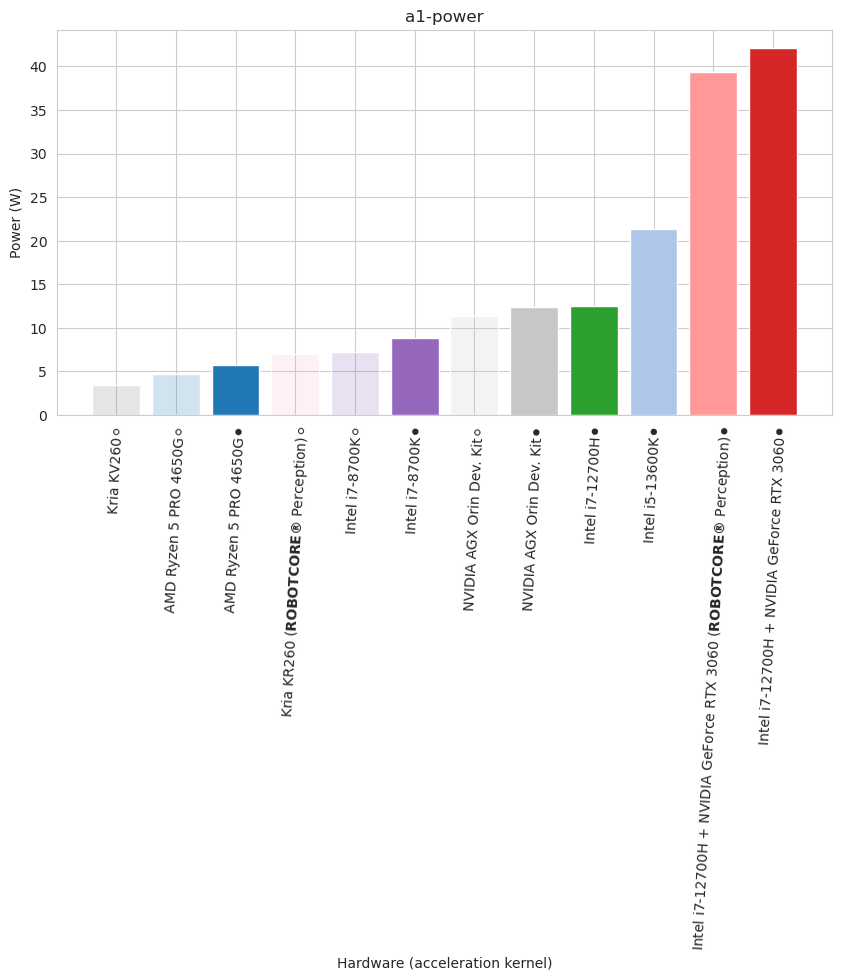}}
\caption{Best power results for \texttt{a1} benchmark.}
\label{subfig:besta1power}
\end{subfigure}
\hfill % ensures that they are side by side
\begin{subfigure}[t]{0.32\textwidth}
\centering
\raisebox{-\height}{\includegraphics[width=\textwidth]{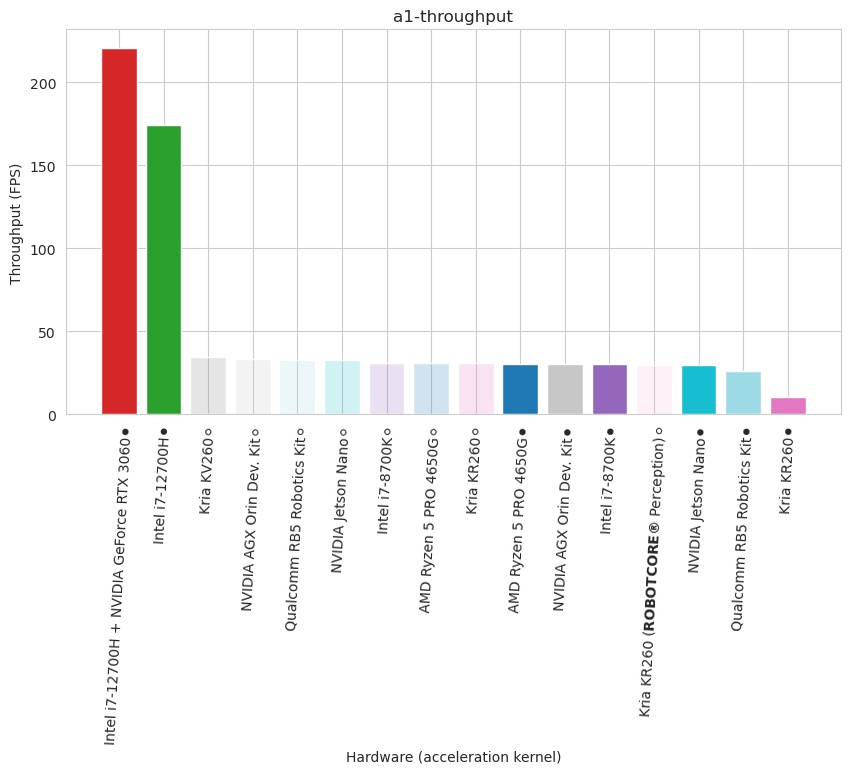}}
\caption{Best throughput results for \texttt{a1} benchmark.}
\label{subfig:besta1throughput}
\end{subfigure}

\hfill

% a2
\begin{subfigure}[t]{0.32\textwidth}  
\centering
\raisebox{-\height}{\includegraphics[width=\textwidth]{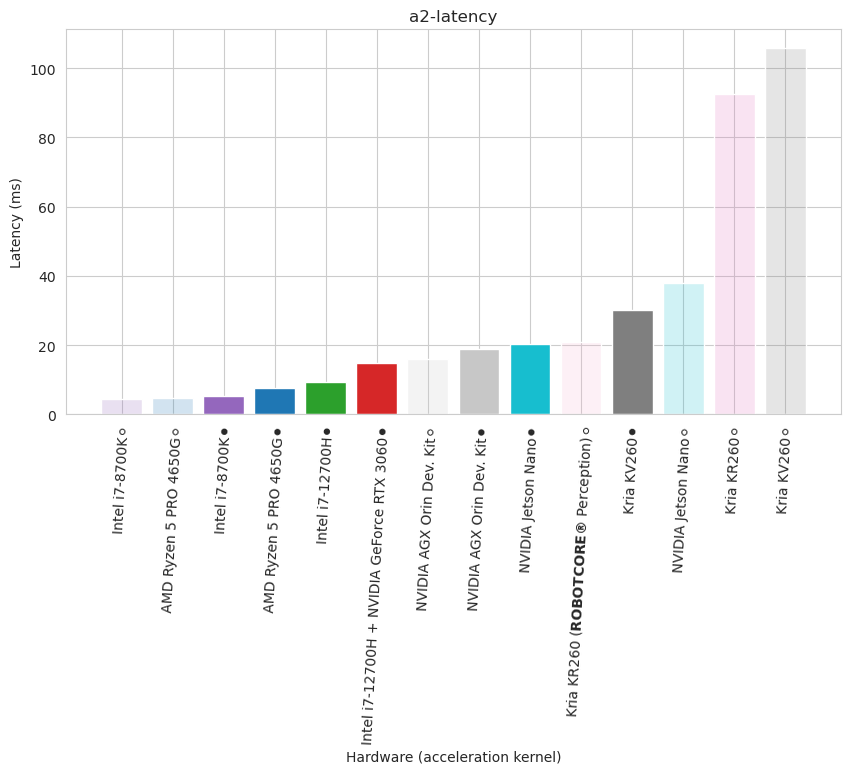}}
\caption{Best latency results for \texttt{a2} benchmark.}
\label{subfig:a8greyboxgraph}
\end{subfigure}
\hfill % ensures that they are side by side
\begin{subfigure}[t]{0.32\textwidth}
\centering
\raisebox{-\height}{\includegraphics[width=\textwidth]{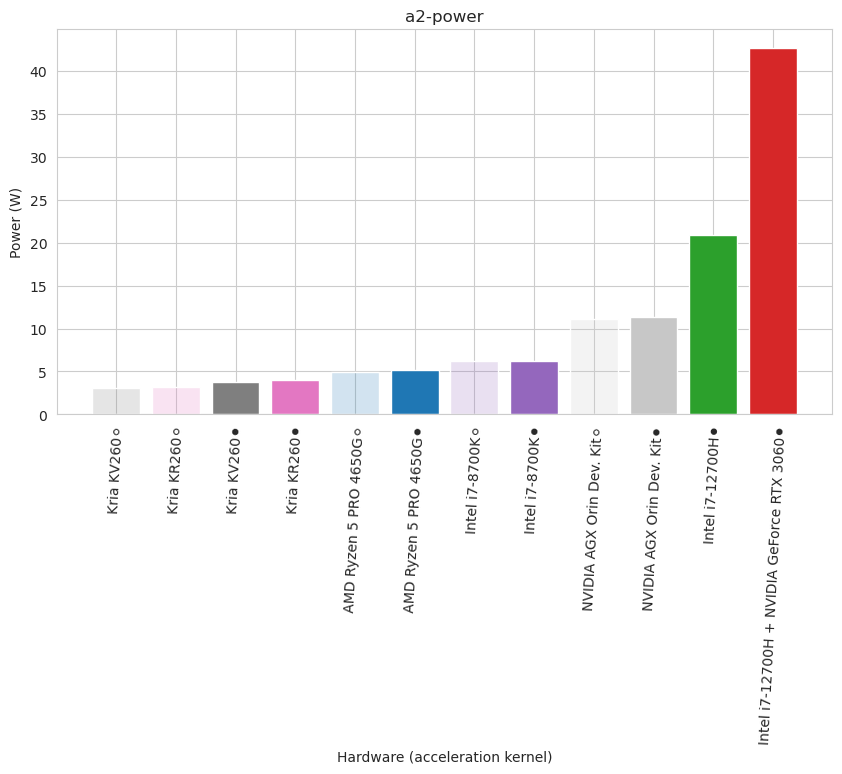}}
\caption{Best power results for \texttt{a2} benchmark.}
\label{subfig:a8blackboxgraph}
\end{subfigure}
\hfill % ensures that they are side by side
\begin{subfigure}[t]{0.32\textwidth}
\centering
\raisebox{-\height}{\includegraphics[width=\textwidth]{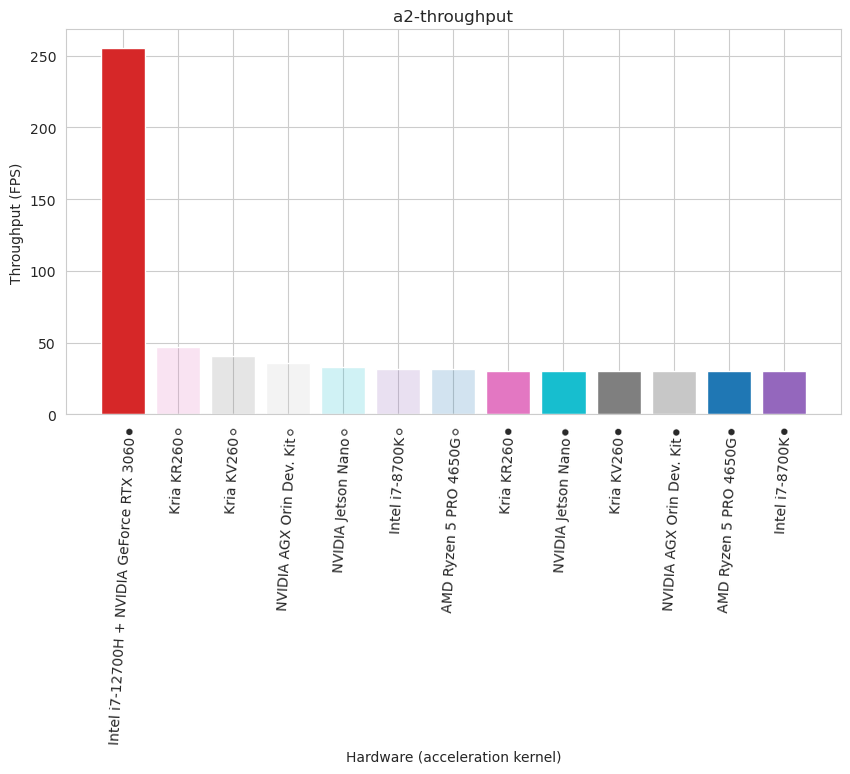}}
\caption{Best throughput results for \texttt{a2} benchmark.}
\label{subfig:a8blackboxgraph}
\end{subfigure}

% a3
\begin{subfigure}[t]{0.32\textwidth}  
\centering
\raisebox{-\height}{\includegraphics[width=\textwidth]{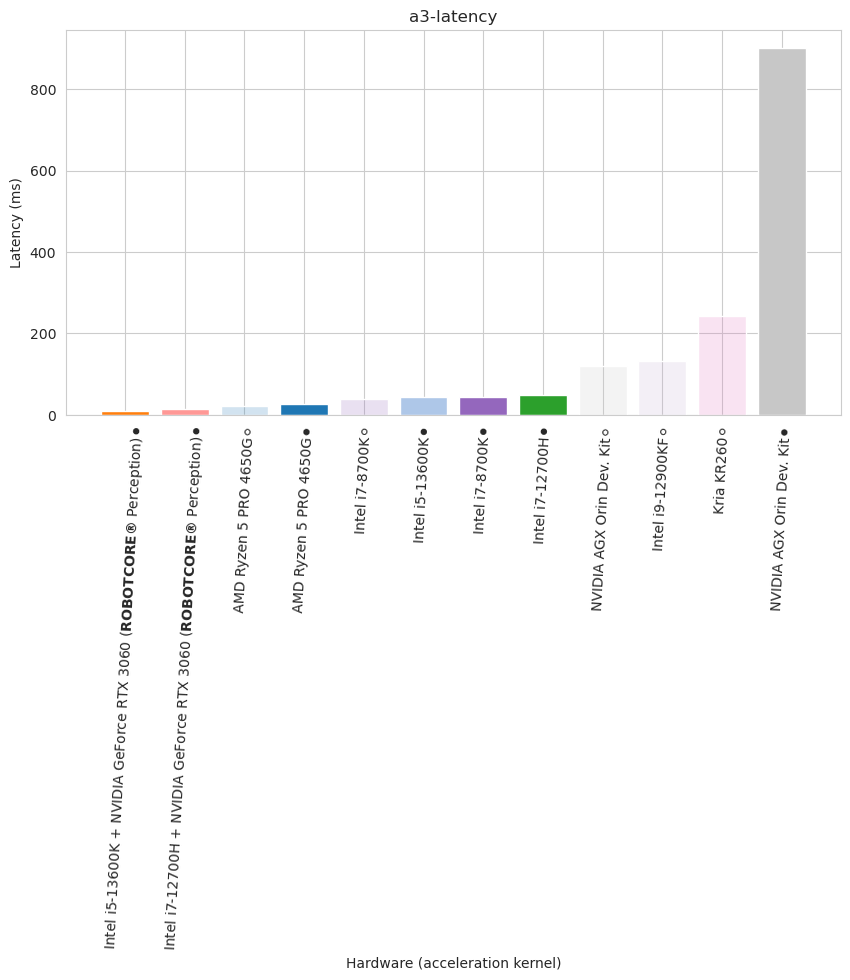}}
\caption{Best latency results for \texttt{a3} benchmark.}
\label{subfig:a8greyboxgraph}
\end{subfigure}
\hfill % ensures that they are side by side
\begin{subfigure}[t]{0.32\textwidth}
\centering
\raisebox{-\height}{\includegraphics[width=\textwidth]{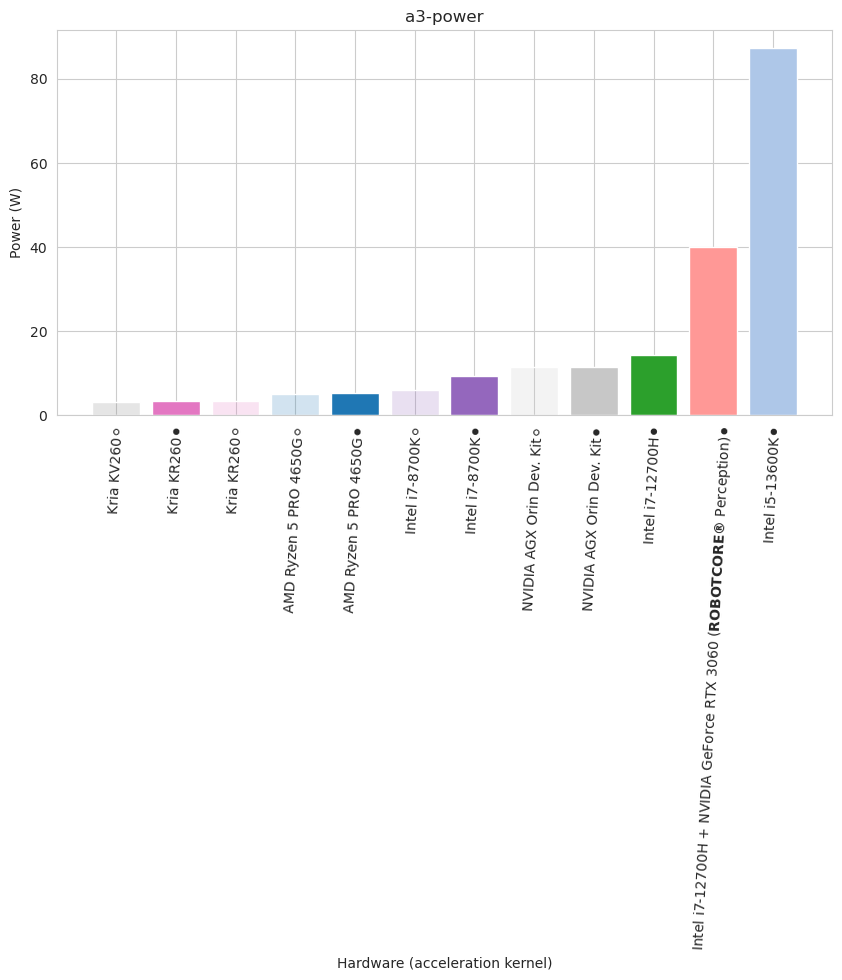}}
\caption{Best power results for \texttt{a3} benchmark.}
\label{subfig:a8blackboxgraph}
\end{subfigure}
\hfill % ensures that they are side by side
\begin{subfigure}[t]{0.32\textwidth}
\centering
\raisebox{-\height}{\includegraphics[width=\textwidth]{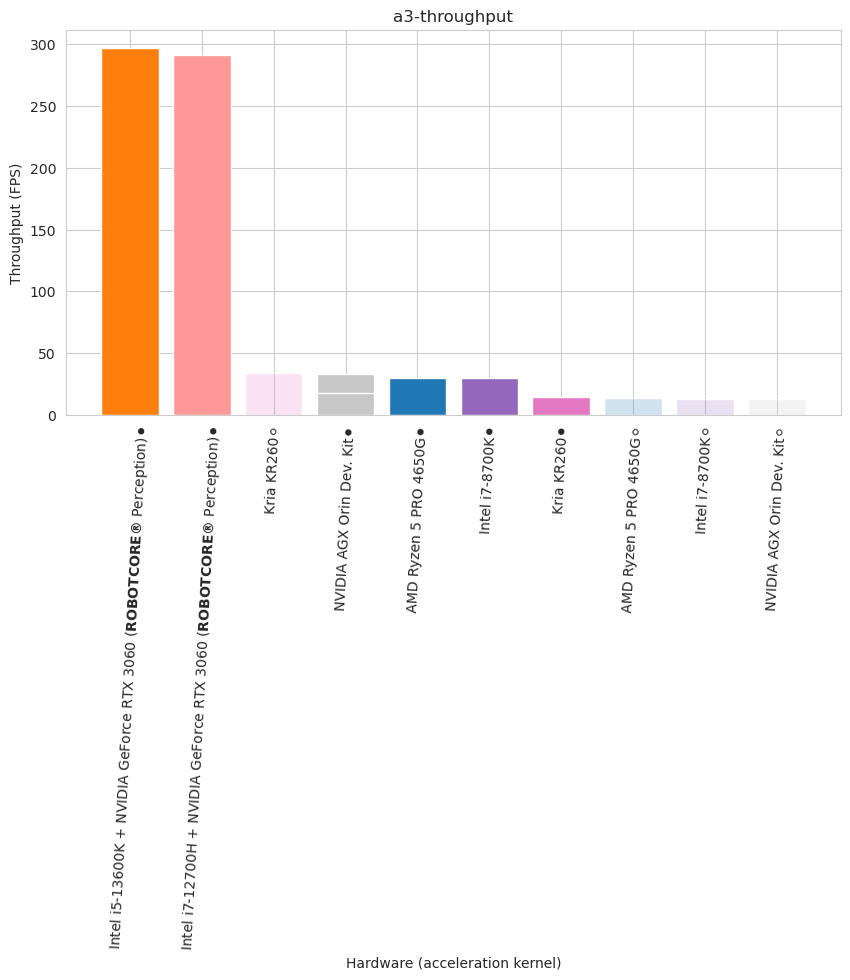}}
\caption{Best throughput results for \texttt{a3} benchmark.}
\label{subfig:a8blackboxgraph}
\end{subfigure}
\caption{Best benchmark results for robot perception \texttt{a1}, \texttt{a2} and \texttt{a3}.}
\label{fig:benchmarks_perception_a1_a3}
\end{figure*}

\begin{figure*}[tbp]
\centering

% a4
\begin{subfigure}[t]{0.32\textwidth}  
\centering
\raisebox{-\height}{\includegraphics[width=\textwidth]{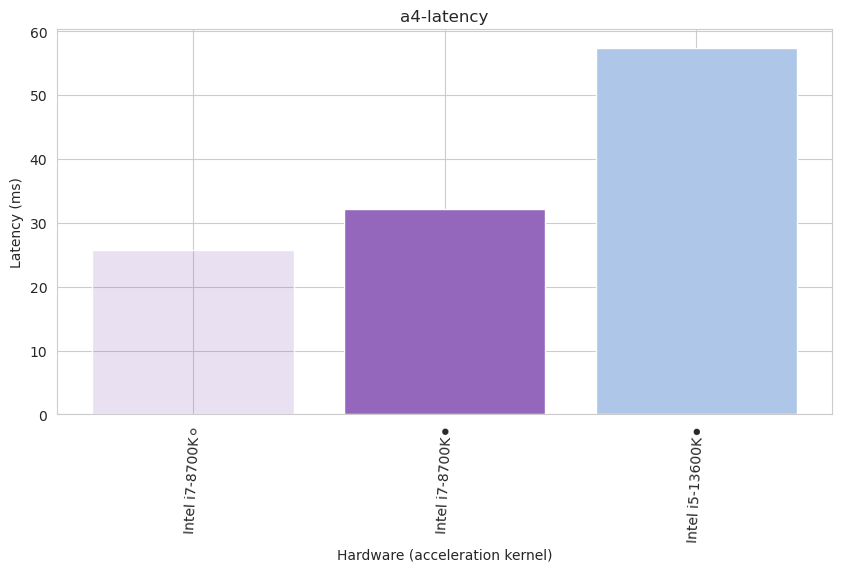}}
\caption{Best latency results for \texttt{a4} benchmark.}
\label{subfig:a8greyboxgraph}
\end{subfigure}
\hfill % ensures that they are side by side
\begin{subfigure}[t]{0.32\textwidth}
\centering
\raisebox{-\height}{\includegraphics[width=\textwidth]{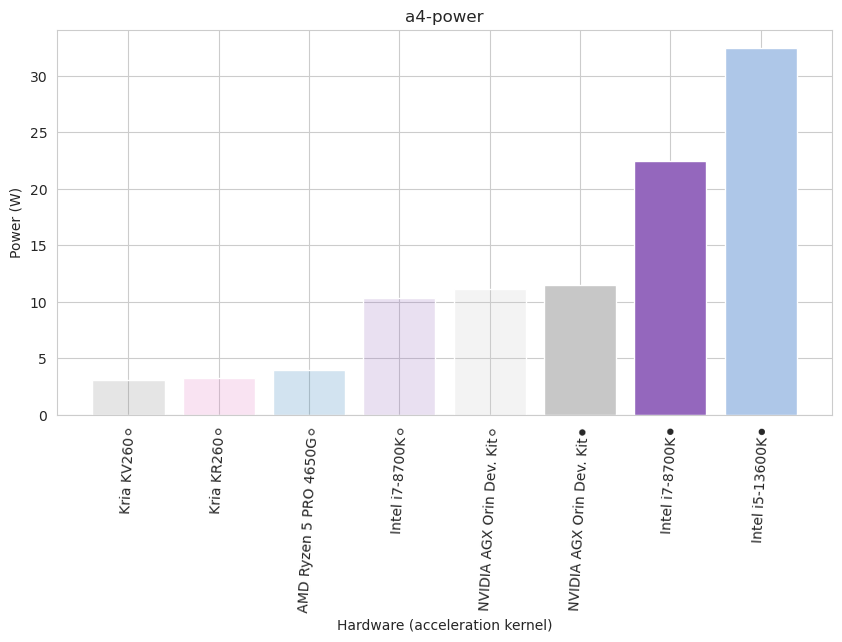}}
\caption{Best power results for \texttt{a4} benchmark.}
\label{subfig:a8blackboxgraph}
\end{subfigure}
\hfill % ensures that they are side by side
\begin{subfigure}[t]{0.32\textwidth}
\centering
\raisebox{-\height}{\includegraphics[width=\textwidth]{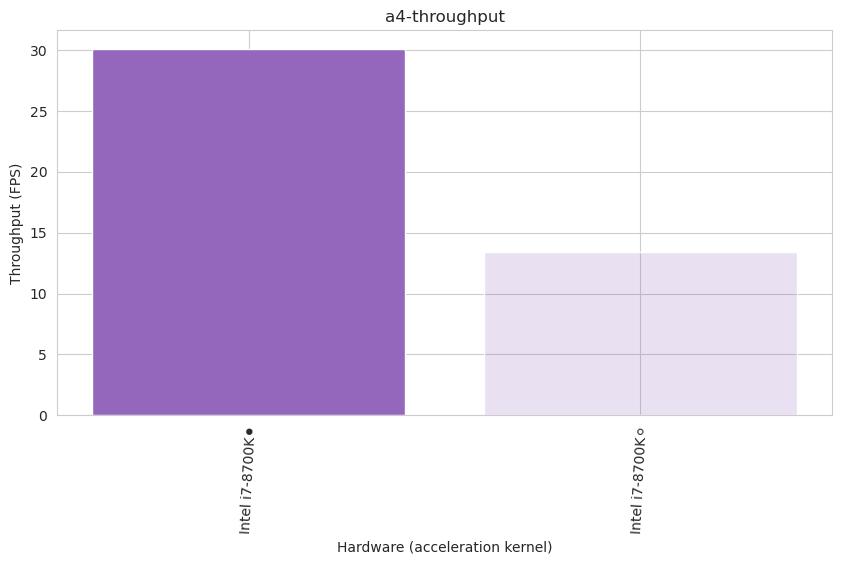}}
\caption{Best throughput results for \texttt{a4} benchmark.}
\label{subfig:a8blackboxgraph}
\end{subfigure}

% a5
\begin{subfigure}[t]{0.32\textwidth}  
\centering
\raisebox{-\height}{\includegraphics[width=\textwidth]{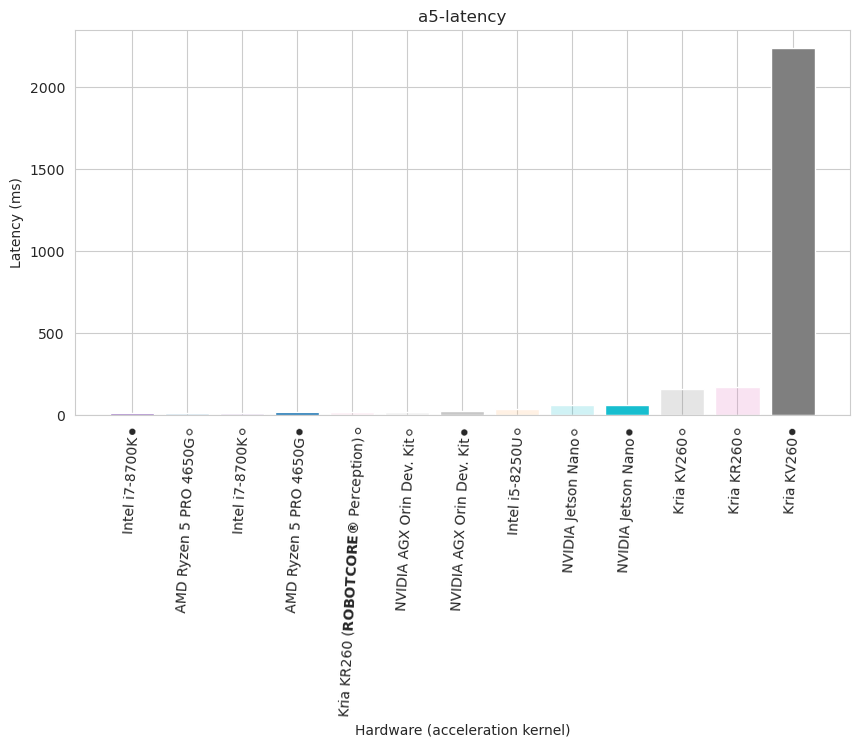}}
\caption{Best latency results for \texttt{a5} benchmark.}
\label{subfig:a8greyboxgraph}
\end{subfigure}
\hfill % ensures that they are side by side
\begin{subfigure}[t]{0.32\textwidth}
\centering
\raisebox{-\height}{\includegraphics[width=\textwidth]{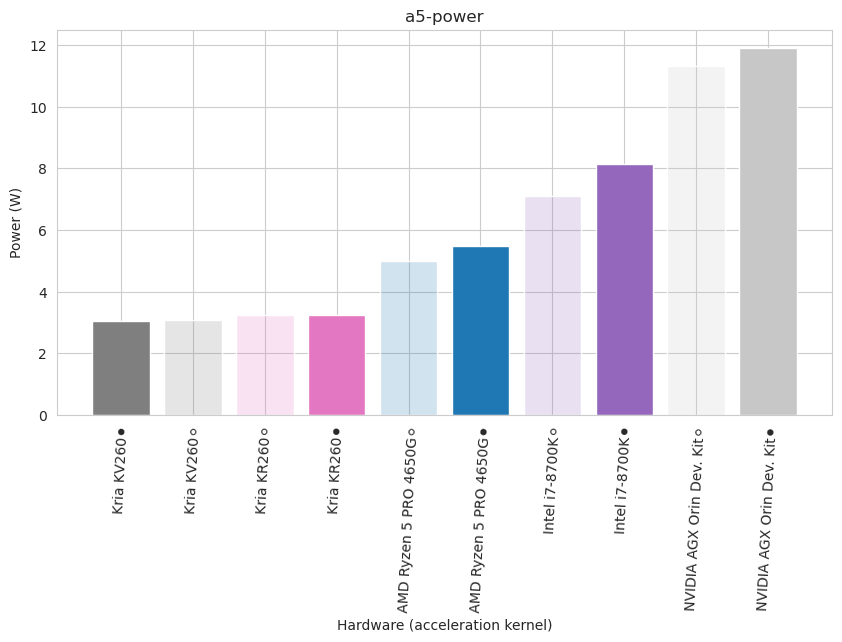}}
\caption{Best power results for \texttt{a5} benchmark.}
\label{subfig:a8blackboxgraph}
\end{subfigure}
\hfill % ensures that they are side by side
\begin{subfigure}[t]{0.32\textwidth}
\centering
\raisebox{-\height}{\includegraphics[width=\textwidth]{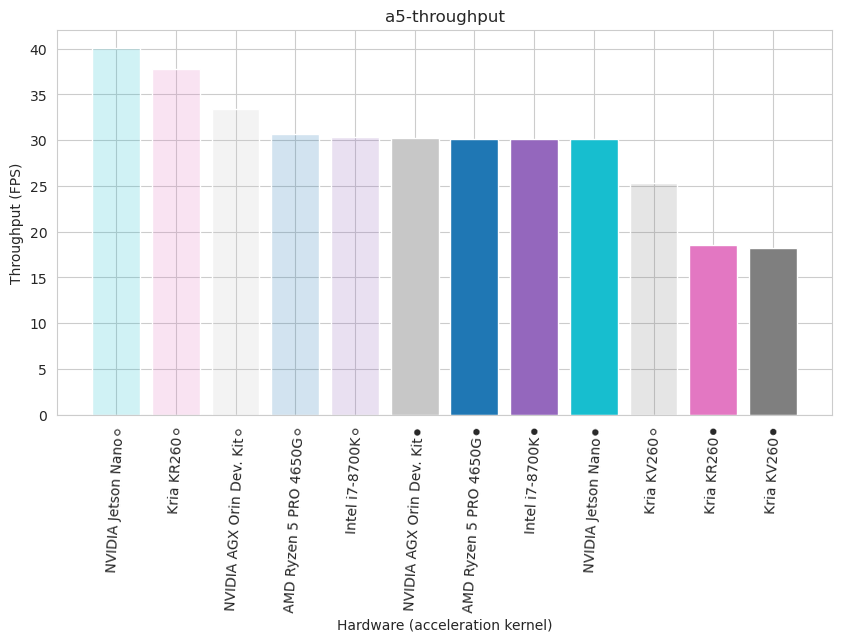}}
\caption{Best throughput results for \texttt{a5} benchmark.}
\label{subfig:a8blackboxgraph}
\end{subfigure}

\caption{Best benchmark results for robot perception \texttt{a4} and \texttt{a5}.}
\label{fig:benchmarks_perception_a4_a5}

\end{figure*}

%%%%%%%%%%%%%%%%%%
%%%%%%%%%%%%%%%%%%%%%%%%%%%%%%%%%%%%%%%%%%%%%%%%%%%%%%%%%%%%%%%%%
%\subsection*{Robotic Localization Benchmarks}
\label{sec:appendix_localization}

\begin{figure*}[tbp]
\centering

% b1
\begin{subfigure}[t]{0.32\textwidth}  
\centering
\raisebox{-\height}{\includegraphics[width=\textwidth]{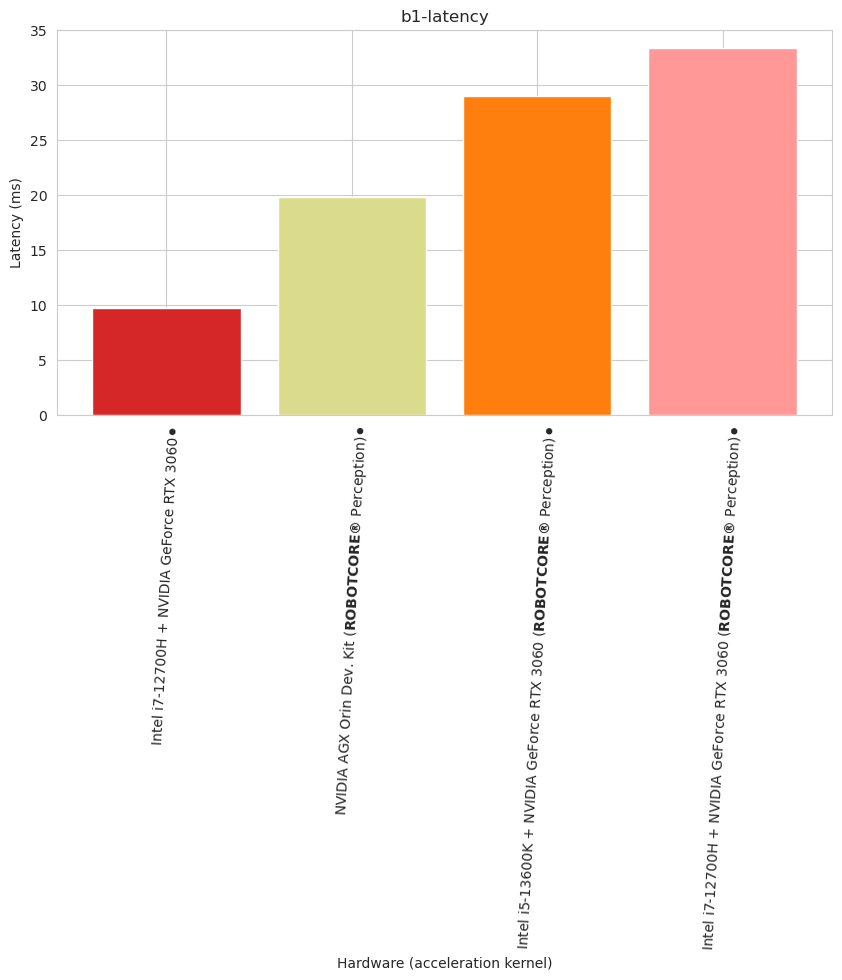}}
\caption{Best latency results for \texttt{b1} benchmark.}
\label{subfig:a8greyboxgraph}
\end{subfigure}
\hfill % ensures that they are side by side
\begin{subfigure}[t]{0.32\textwidth}
\centering
\raisebox{-\height}{\includegraphics[width=\textwidth]{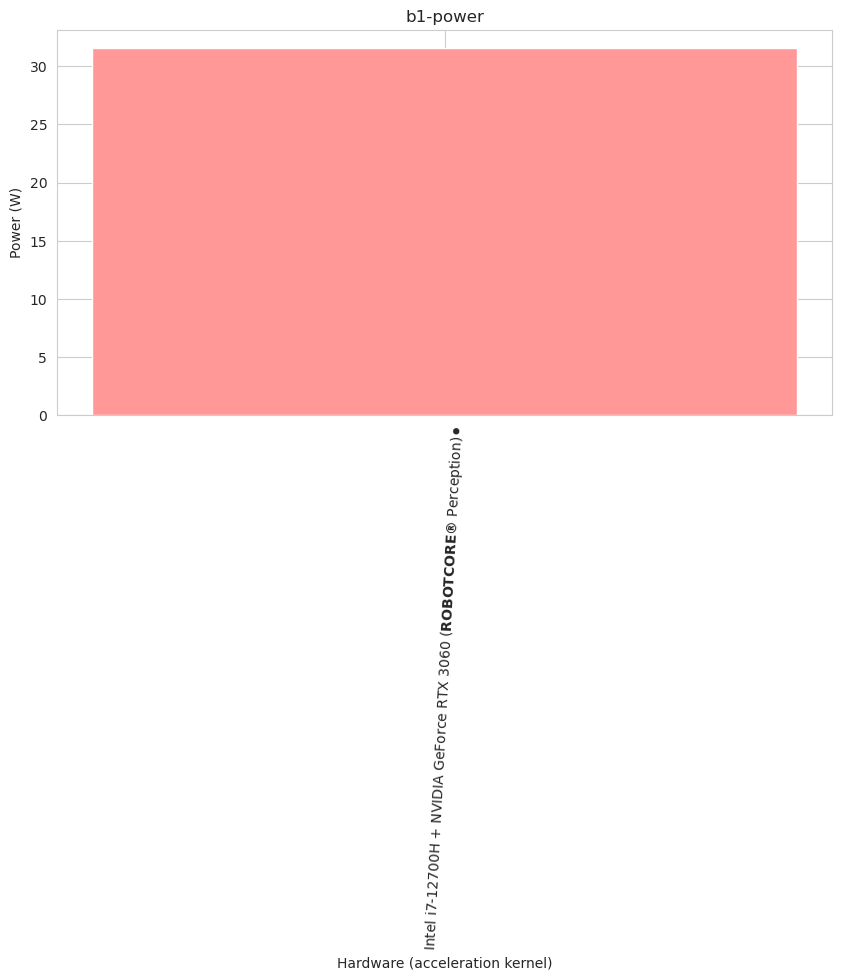}}
\caption{Best power results for \texttt{b1} benchmark.}
\label{subfig:a8blackboxgraph}
\end{subfigure}
\hfill % ensures that they are side by side
\begin{subfigure}[t]{0.32\textwidth}
\centering
\raisebox{-\height}{\includegraphics[width=\textwidth]{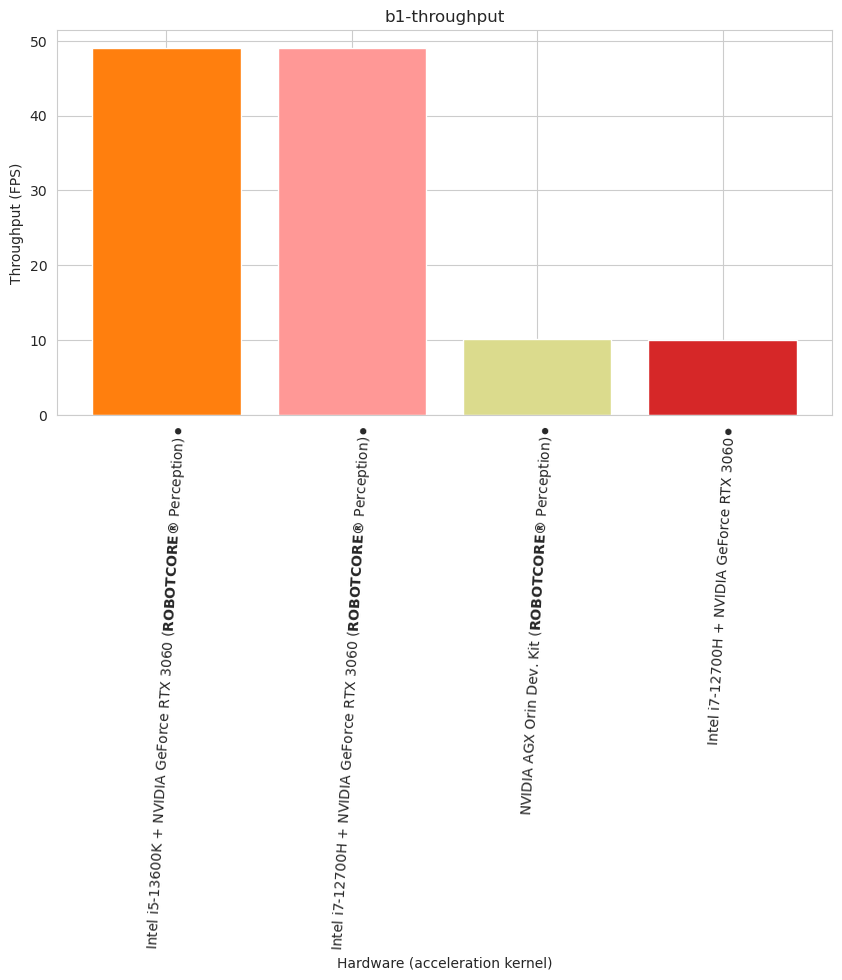}}
\caption{Best throughput results for \texttt{b1} benchmark.}
\label{subfig:a8blackboxgraph}
\end{subfigure}

\hfill

% b2
\begin{subfigure}[t]{0.32\textwidth}  
\centering
\raisebox{-\height}{\includegraphics[width=\textwidth]{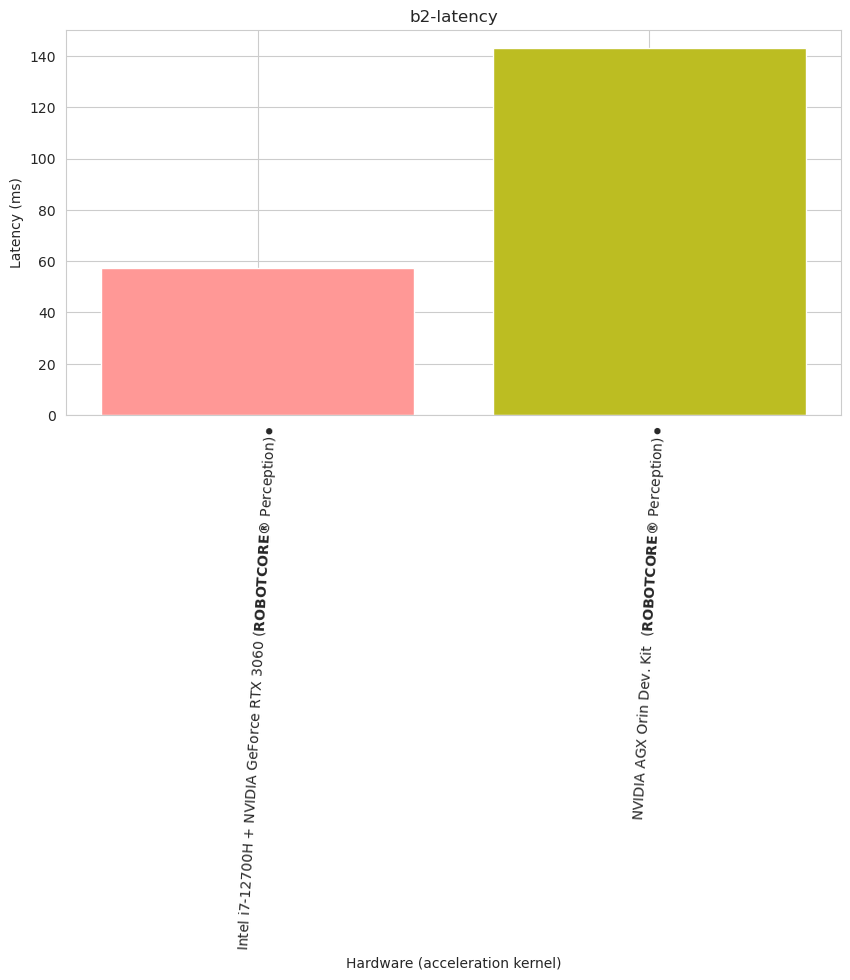}}
\caption{Best latency results for \texttt{b2} benchmark.}
\label{subfig:a8greyboxgraph}
\end{subfigure}
\hfill % ensures that they are side by side
\begin{subfigure}[t]{0.32\textwidth}
\centering
\raisebox{-\height}{\includegraphics[width=\textwidth]{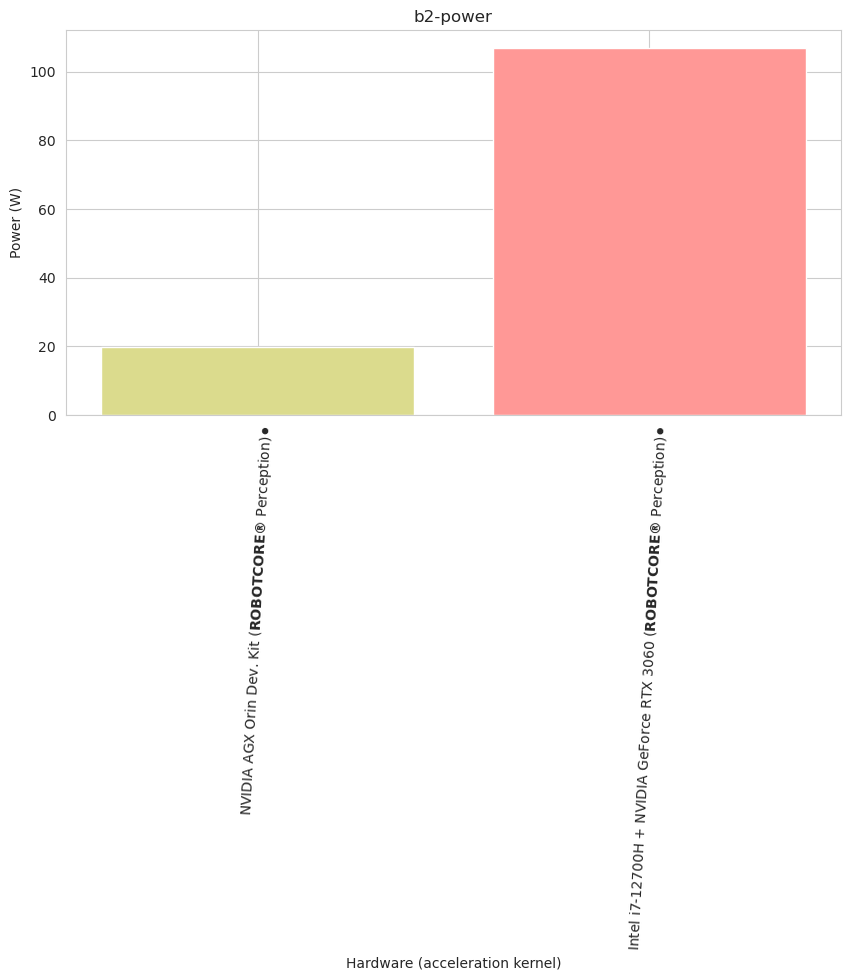}}
\caption{Best power results for \texttt{b2} benchmark.}
\label{subfig:a8blackboxgraph}
\end{subfigure}
\hfill % ensures that they are side by side
\begin{subfigure}[t]{0.32\textwidth}
\centering
\raisebox{-\height}{\includegraphics[width=\textwidth]{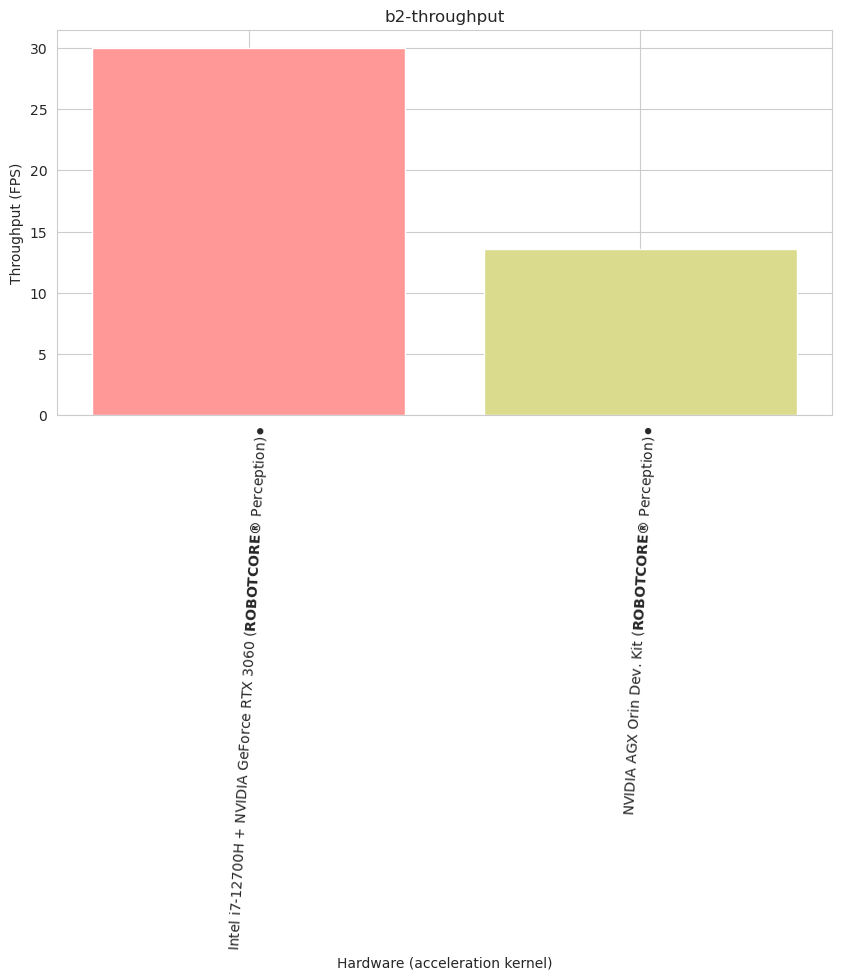}}
\caption{Best throughput results for \texttt{b2} benchmark.}
\label{subfig:a8blackboxgraph}
\end{subfigure}

% b3
\begin{subfigure}[t]{0.32\textwidth}  
\centering
\raisebox{-\height}{\includegraphics[width=\textwidth]{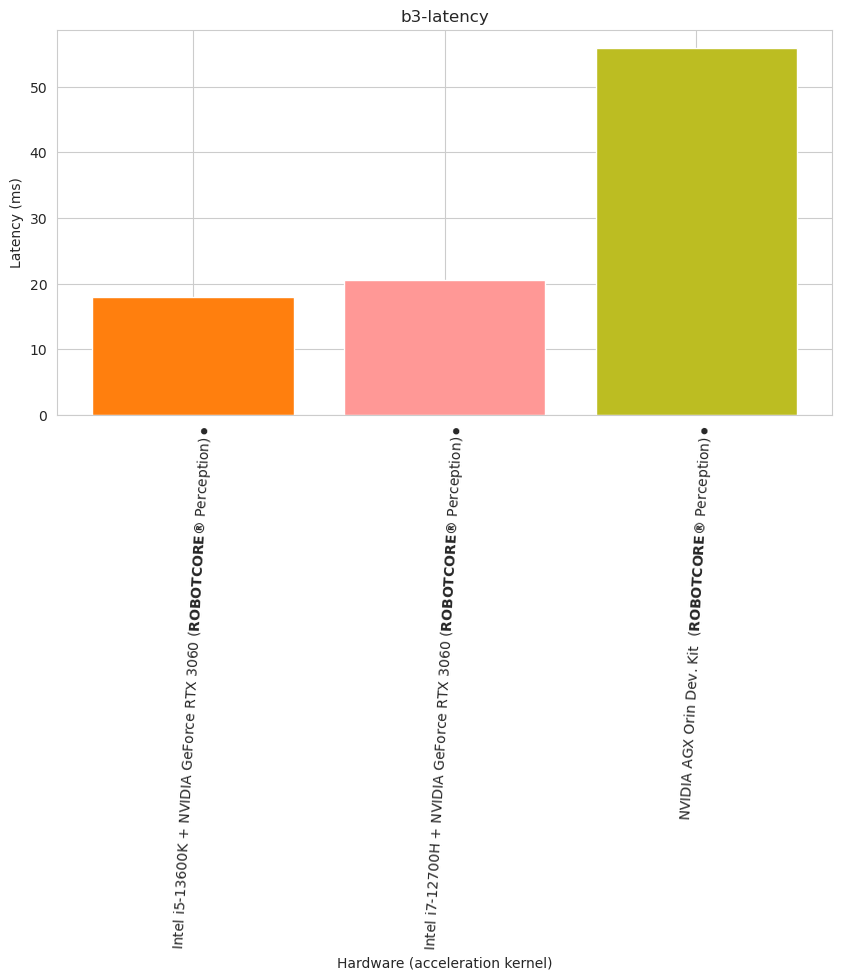}}
\caption{Best latency results for \texttt{b3} benchmark.}
\label{subfig:a8greyboxgraph}
\end{subfigure}
\hfill % ensures that they are side by side
\begin{subfigure}[t]{0.32\textwidth}
\centering
\raisebox{-\height}{\includegraphics[width=\textwidth]{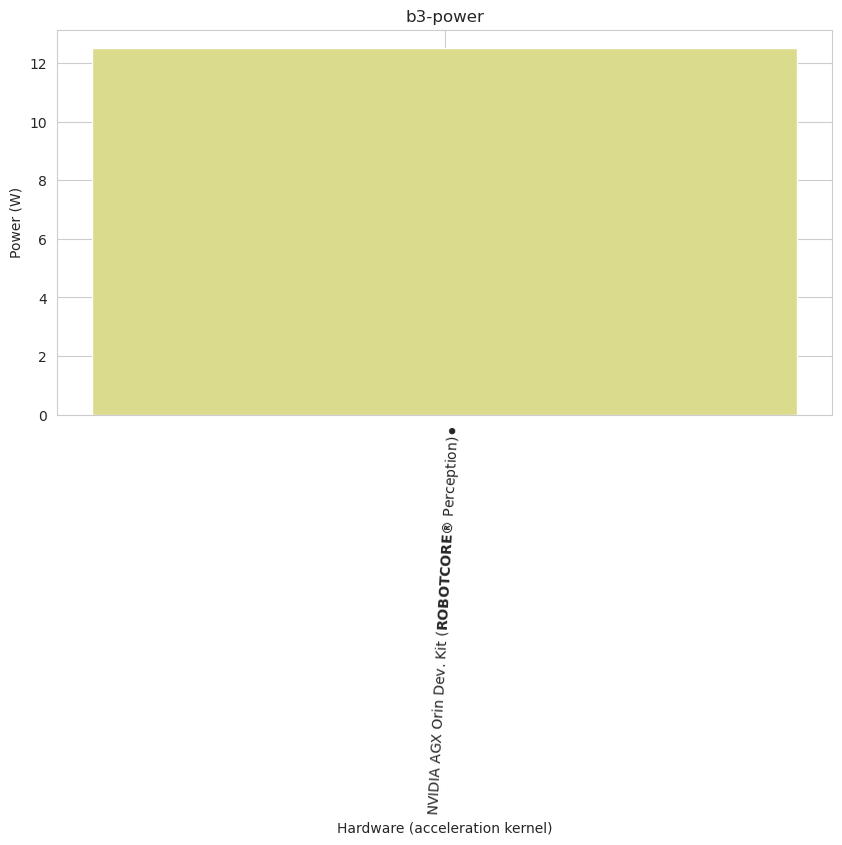}}
\caption{Best power results for \texttt{b3} benchmark.}
\label{subfig:a8blackboxgraph}
\end{subfigure}
\hfill % ensures that they are side by side
\begin{subfigure}[t]{0.32\textwidth}
\centering
\raisebox{-\height}{\includegraphics[width=\textwidth]{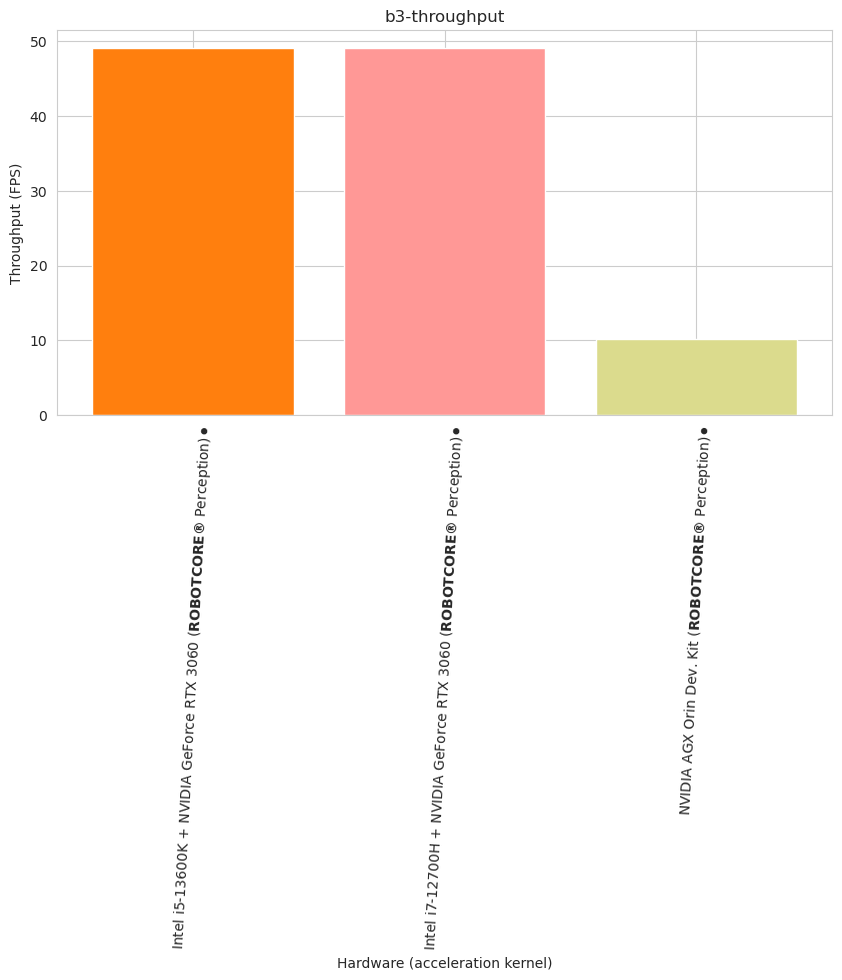}}
\caption{Best throughput results for \texttt{b3} benchmark.}
\label{subfig:a8blackboxgraph}
\end{subfigure}
\caption{Best benchmark results for robot localization \texttt{b1}, \texttt{b2} and \texttt{b3}.}
\label{fig:benchmarks_perception_b1_b3}
\end{figure*}

%%%%%%%%%%%%%%%%%%%%%%%%%%%%%%%%%%%%%%%%%%%%%%%%%%%%%%%%%%%%%%%%%
%\subsection*{Robotic Control Benchmarks}
\label{sec:appendix_control}

\begin{figure*}[tbp]
\centering
    
% c1
\begin{subfigure}[t]{0.32\textwidth}  
\centering
\raisebox{-\height}{\includegraphics[width=\textwidth]{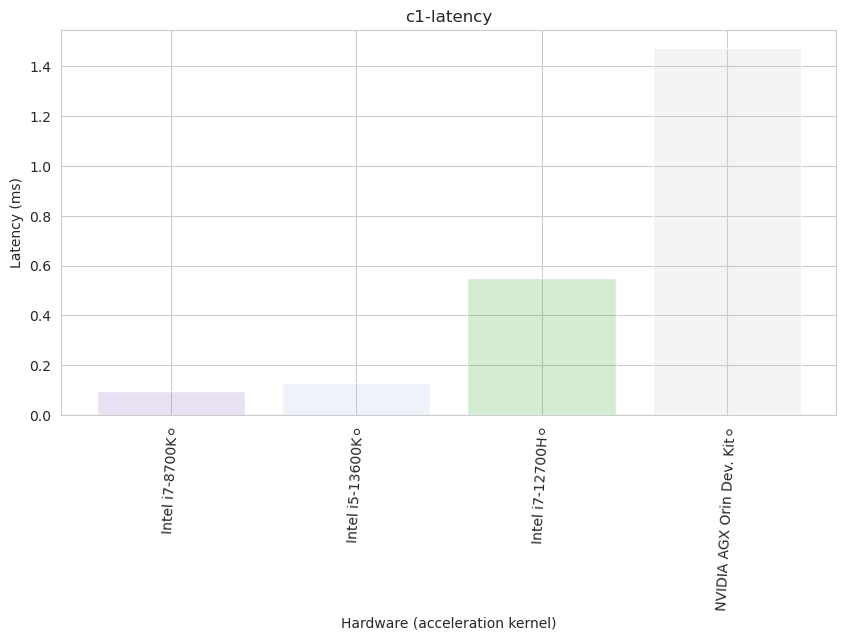}}
\caption{Best latency results for \texttt{c1} benchmark.}
\label{subfig:a8greyboxgraph}
\end{subfigure}
\hfill % ensures that they are side by side
\begin{subfigure}[t]{0.32\textwidth}
\centering
\raisebox{-\height}{\includegraphics[width=\textwidth]{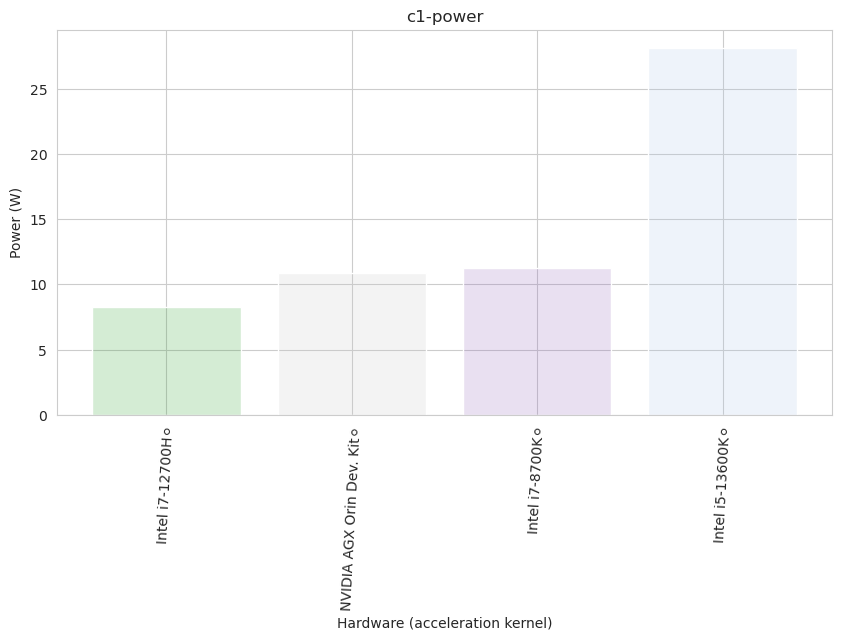}}
\caption{Best power results for \texttt{c1} benchmark.}
\label{subfig:a8blackboxgraph}
\end{subfigure}
\hfill % ensures that they are side by side
\begin{subfigure}[t]{0.32\textwidth}
\centering
\raisebox{-\height}{\includegraphics[width=\textwidth]{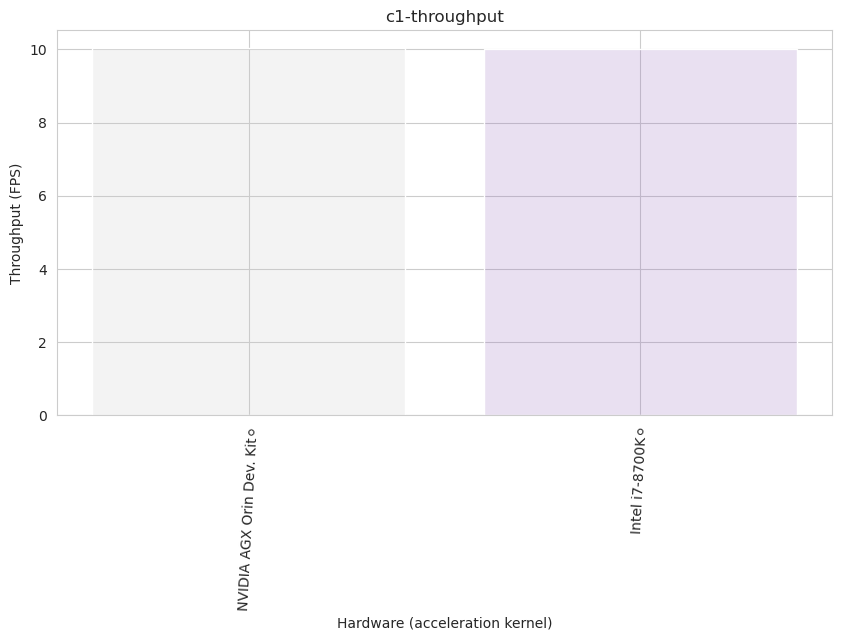}}
\caption{Best throughput results for \texttt{c1} benchmark.}
\label{subfig:a8blackboxgraph}
\end{subfigure}

\hfill

% c2
\begin{subfigure}[t]{0.32\textwidth}  
\centering
\raisebox{-\height}{\includegraphics[width=\textwidth]{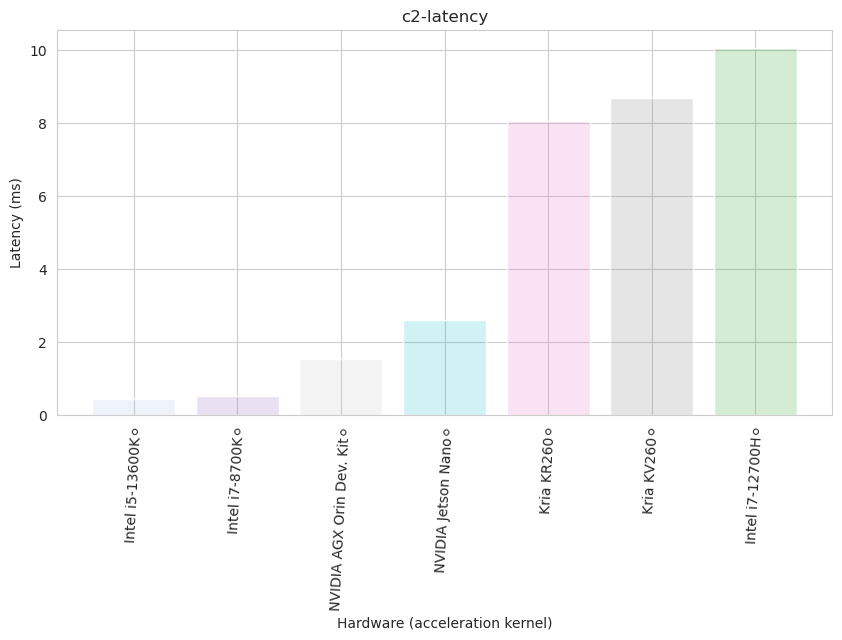}}
\caption{Best latency results for \texttt{c2} benchmark.}
\label{subfig:a8greyboxgraph}
\end{subfigure}
\hfill % ensures that they are side by side
\begin{subfigure}[t]{0.32\textwidth}
\centering
\raisebox{-\height}{\includegraphics[width=\textwidth]{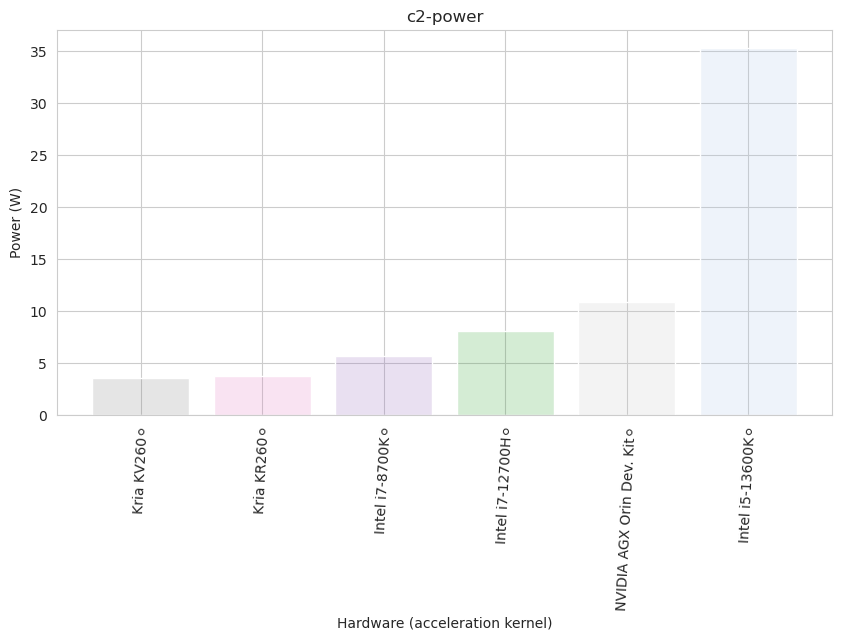}}
\caption{Best power results for \texttt{c2} benchmark.}
\label{subfig:a8blackboxgraph}
\end{subfigure}
\hfill % ensures that they are side by side
\begin{subfigure}[t]{0.32\textwidth}
\centering
\raisebox{-\height}{\includegraphics[width=\textwidth]{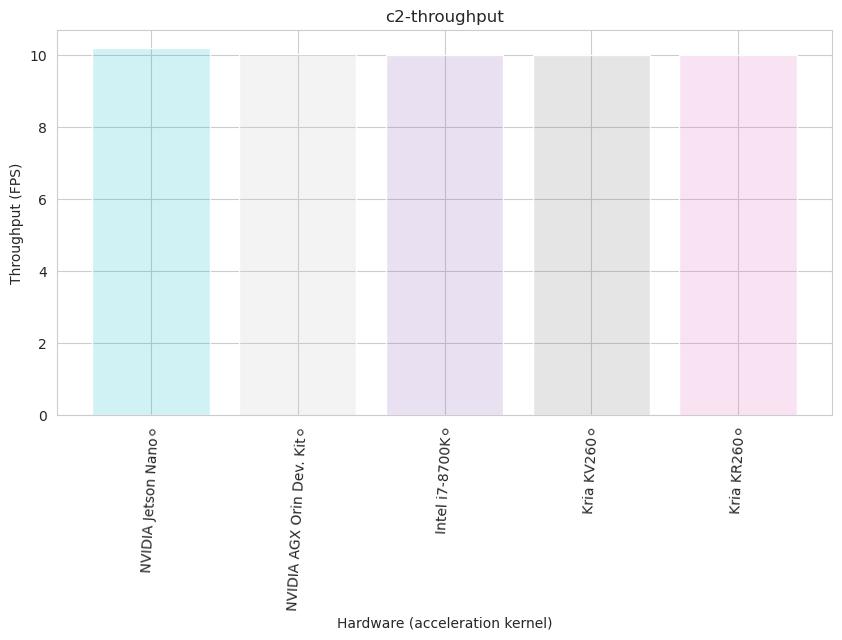}}
\caption{Best throughput results for \texttt{c2} benchmark.}
\label{subfig:a8blackboxgraph}
\end{subfigure}

% c3
\begin{subfigure}[t]{0.32\textwidth}  
\centering
\raisebox{-\height}{\includegraphics[width=\textwidth]{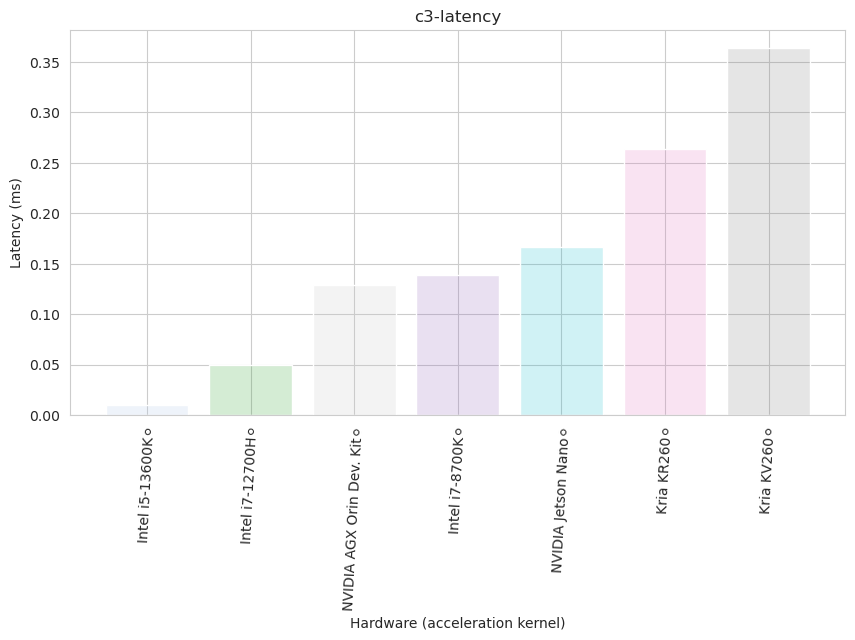}}
\caption{Best latency results for \texttt{c3} benchmark.}
\label{subfig:a8greyboxgraph}
\end{subfigure}
\hfill % ensures that they are side by side
\begin{subfigure}[t]{0.32\textwidth}
\centering
\raisebox{-\height}{\includegraphics[width=\textwidth]{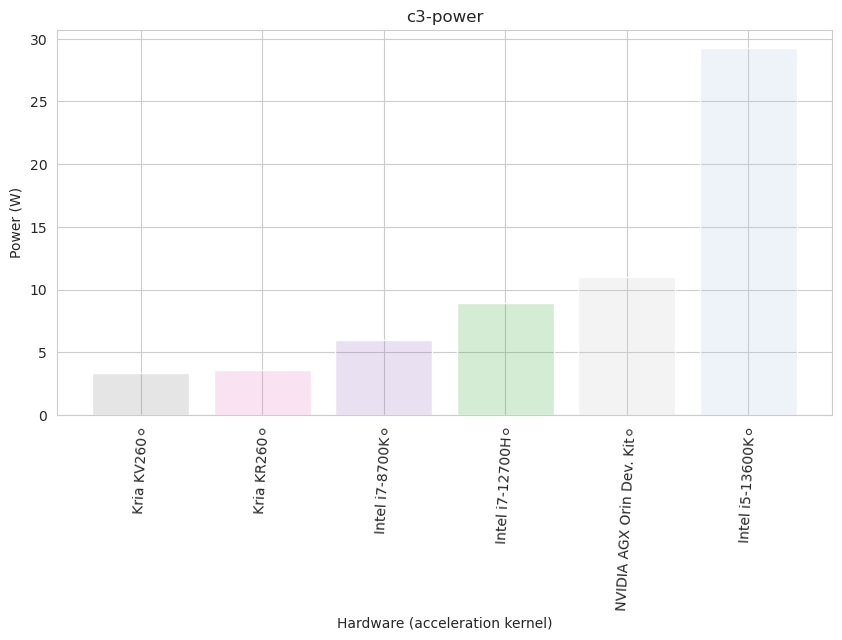}}
\caption{Best power results for \texttt{c3} benchmark.}
\label{subfig:a8blackboxgraph}
\end{subfigure}
\hfill % ensures that they are side by side
\begin{subfigure}[t]{0.32\textwidth}
\centering
\raisebox{-\height}{\includegraphics[width=\textwidth]{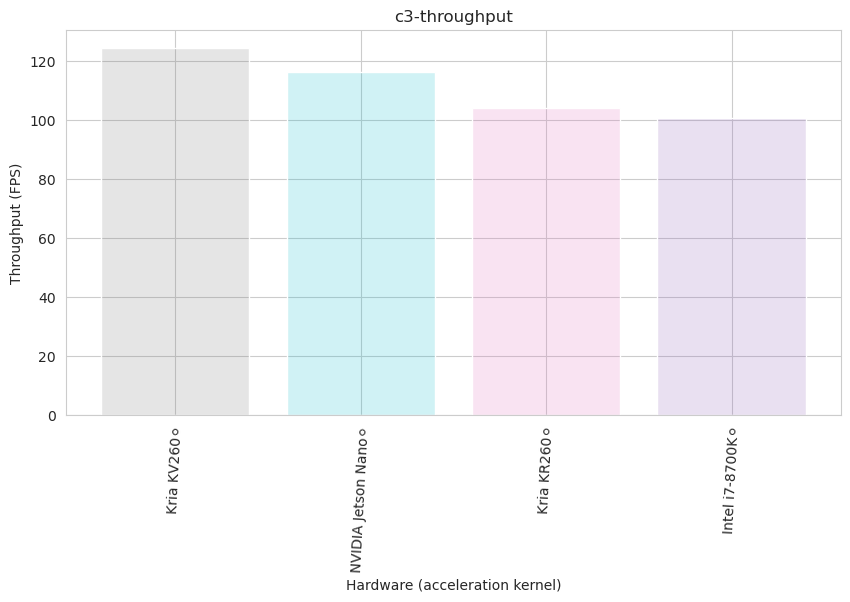}}
\caption{Best throughput results for \texttt{c3} benchmark.}
\label{subfig:a8blackboxgraph}
\end{subfigure}
\caption{Best benchmark results for robot control \texttt{c1}, \texttt{c2} and \texttt{c3}.}
\label{fig:benchmarks_control_c1_c3}
\end{figure*}

\begin{figure*}[tbp]
\centering
    
% c4
\begin{subfigure}[t]{0.32\textwidth}  
\centering
\raisebox{-\height}{\includegraphics[width=\textwidth]{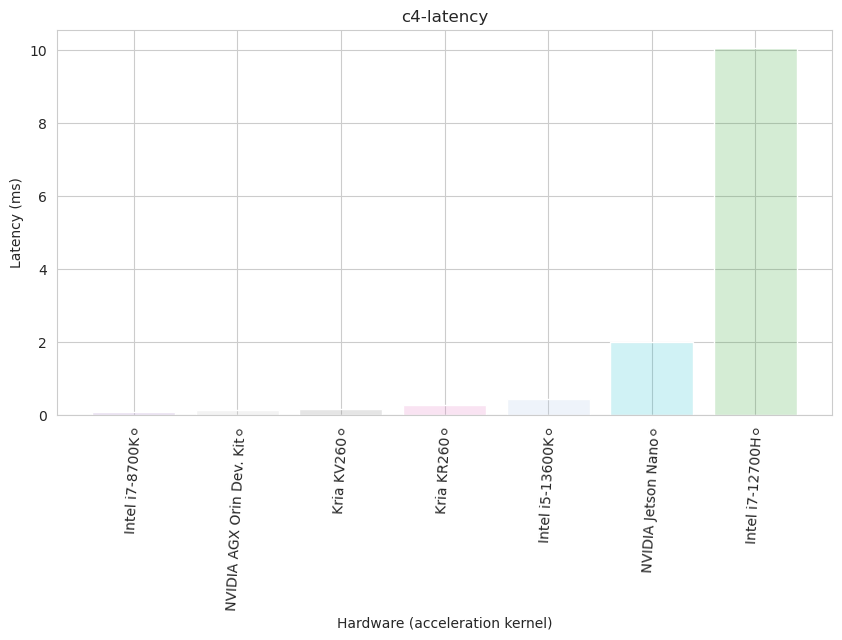}}
\caption{Best latency results for \texttt{c4} benchmark.}
\label{subfig:a8greyboxgraph}
\end{subfigure}
\hfill % ensures that they are side by side
\begin{subfigure}[t]{0.32\textwidth}
\centering
\raisebox{-\height}{\includegraphics[width=\textwidth]{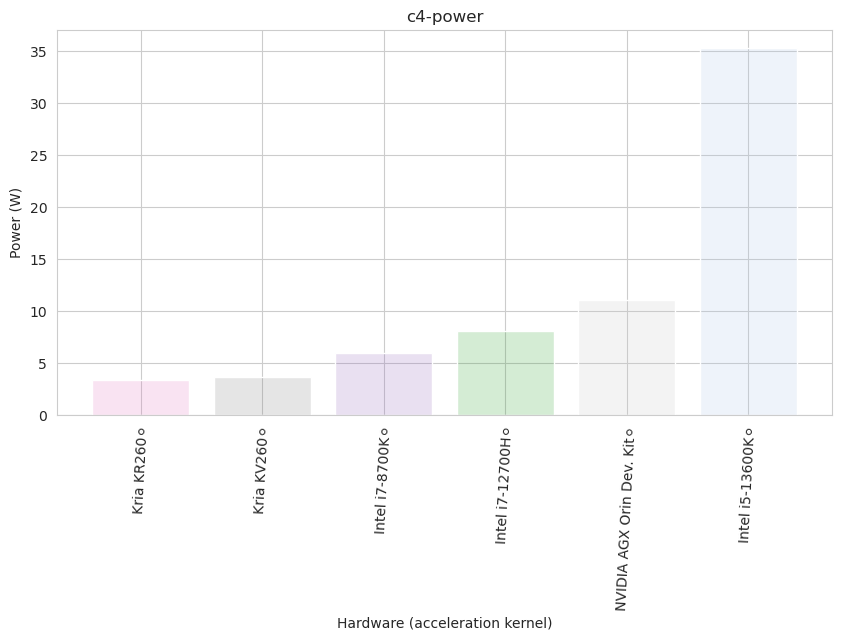}}
\caption{Best power results for \texttt{c4} benchmark.}
\label{subfig:a8blackboxgraph}
\end{subfigure}
\hfill % ensures that they are side by side
\begin{subfigure}[t]{0.32\textwidth}
\centering
\raisebox{-\height}{\includegraphics[width=\textwidth]{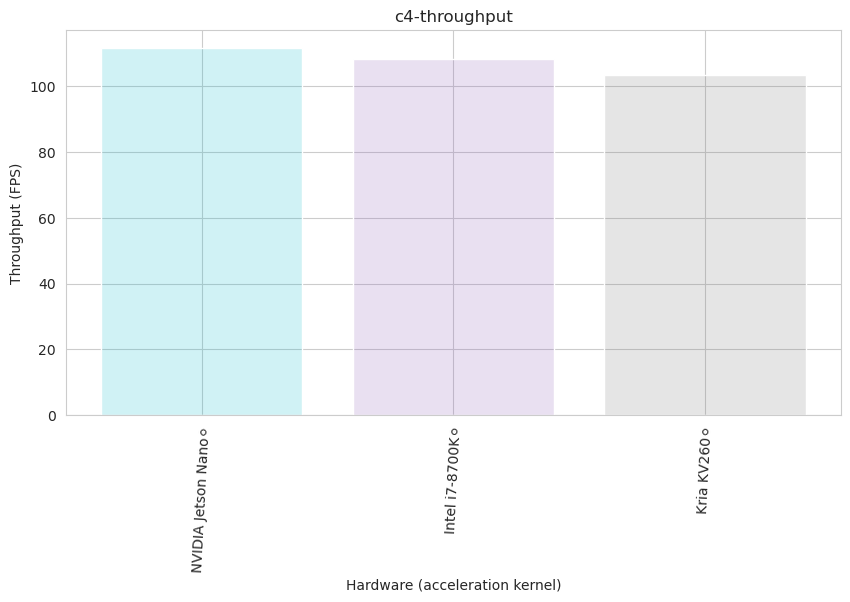}}
\caption{Best throughput results for \texttt{c4} benchmark.}
\label{subfig:a8blackboxgraph}
\end{subfigure}

\hfill

% c5
\begin{subfigure}[t]{0.32\textwidth}  
\centering
\raisebox{-\height}{\includegraphics[width=\textwidth]{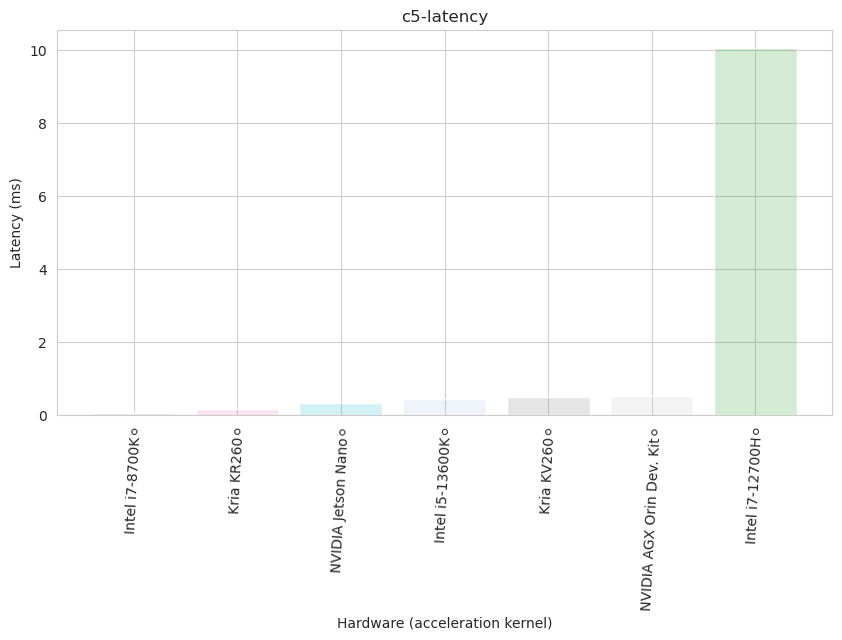}}
\caption{Best latency results for \texttt{c5} benchmark.}
\label{subfig:a8greyboxgraph}
\end{subfigure}
\hfill % ensures that they are side by side
\begin{subfigure}[t]{0.32\textwidth}
\centering
\raisebox{-\height}{\includegraphics[width=\textwidth]{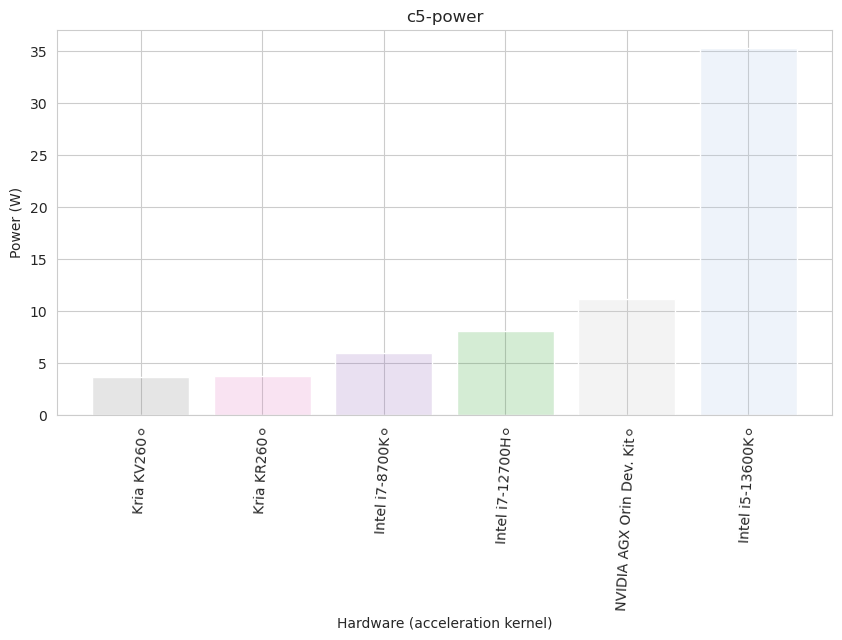}}
\caption{Best power results for \texttt{c5} benchmark.}
\label{subfig:a8blackboxgraph}
\end{subfigure}
\hfill % ensures that they are side by side
\begin{subfigure}[t]{0.32\textwidth}
\centering
\raisebox{-\height}{\includegraphics[width=\textwidth]{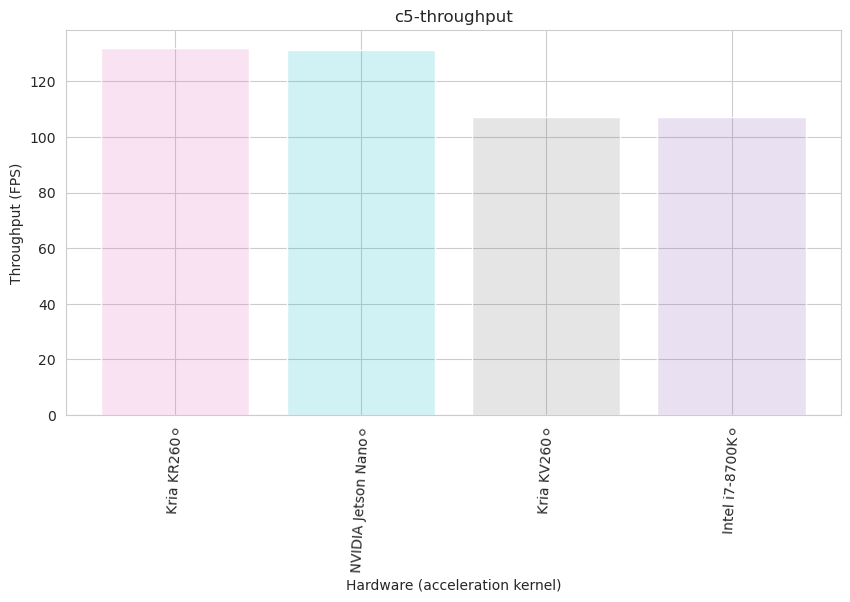}}
\caption{Best throughput results for \texttt{c5} benchmark.}
\label{subfig:a8blackboxgraph}
\end{subfigure}

\caption{Best benchmark results for robot control \texttt{c4} and \texttt{c5}}
\label{fig:benchmarks_control_c4_c3}
\end{figure*}

%%%%%%%%%%%%%%%%%%%%%%%%%%%%%%%%%%%%%%%%%%%%%%%%%%%%%%%%%%%%%%%%%
\label{sec:appendix_manipulation}

\begin{figure*}[tbp]
\centering
    
% d1
\begin{subfigure}[t]{0.32\textwidth}  
\centering
\raisebox{-\height}{\includegraphics[width=\textwidth]{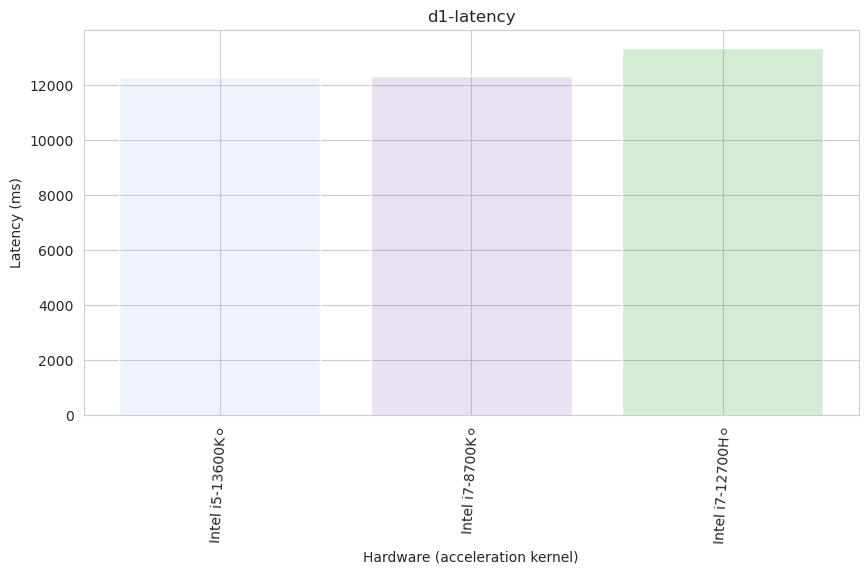}}
\caption{Best latency results for \texttt{d1} benchmark.}
\label{subfig:a8greyboxgraph}
\end{subfigure}
\hfill % ensures that they are side by side
\begin{subfigure}[t]{0.32\textwidth}
\centering
\raisebox{-\height}{\includegraphics[width=\textwidth]{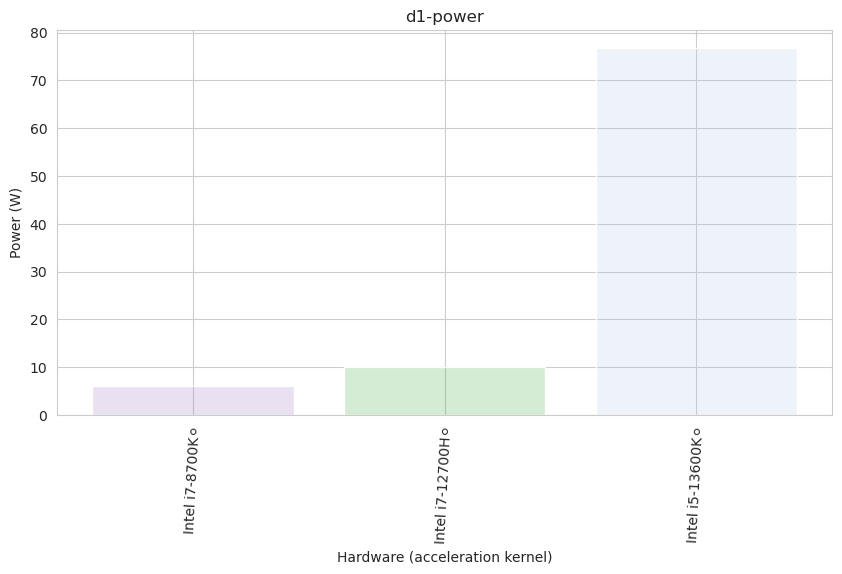}}
\caption{Best power results for \texttt{d1} benchmark.}
\label{subfig:a8blackboxgraph}
\end{subfigure}
\hfill
% d2
\begin{subfigure}[t]{0.32\textwidth}  
\centering
\raisebox{-\height}{\includegraphics[width=\textwidth]{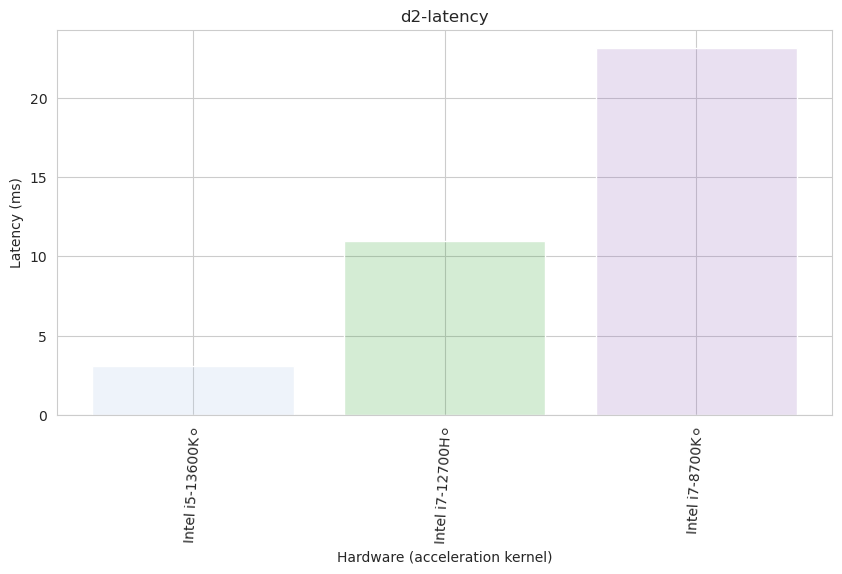}}
\caption{Best latency results for \texttt{d2} benchmark.}
\label{subfig:a8greyboxgraph}
\end{subfigure}
\hfill % ensures that they are side by side
\begin{subfigure}[t]{0.32\textwidth}
\centering
\raisebox{-\height}{\includegraphics[width=\textwidth]{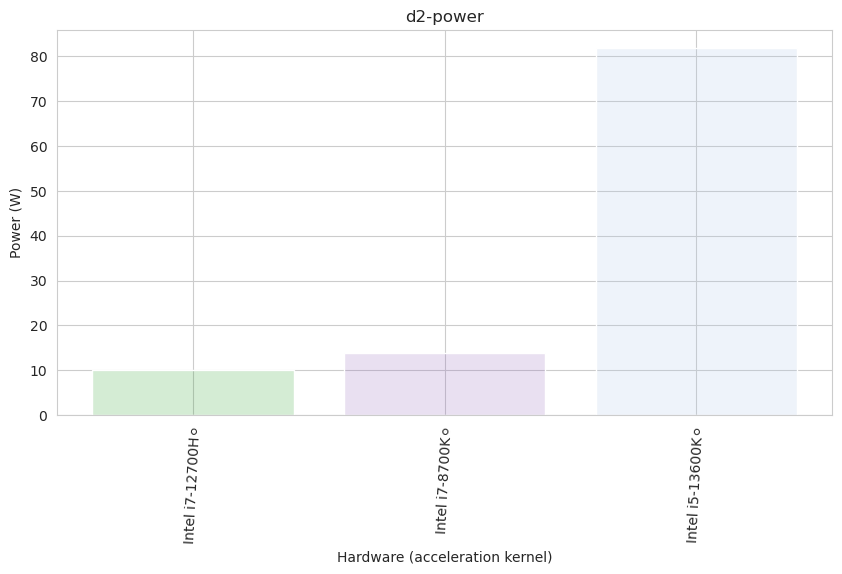}}
\caption{Best power results for \texttt{d2} benchmark.}
\label{subfig:a8blackboxgraph}
\end{subfigure}
\hfill % ensures that they are side by side
% d3
\begin{subfigure}[t]{0.32\textwidth}  
\centering
\raisebox{-\height}{\includegraphics[width=\textwidth]{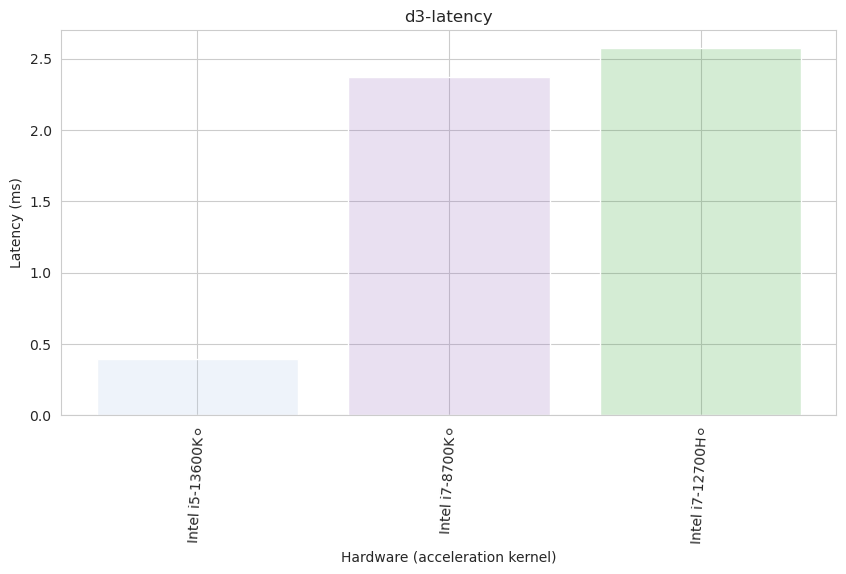}}
\caption{Best latency results for \texttt{d3} benchmark.}
\label{subfig:a8greyboxgraph}
\end{subfigure}
\hfill % ensures that they are side by side
\begin{subfigure}[t]{0.32\textwidth}
\centering
\raisebox{-\height}{\includegraphics[width=\textwidth]{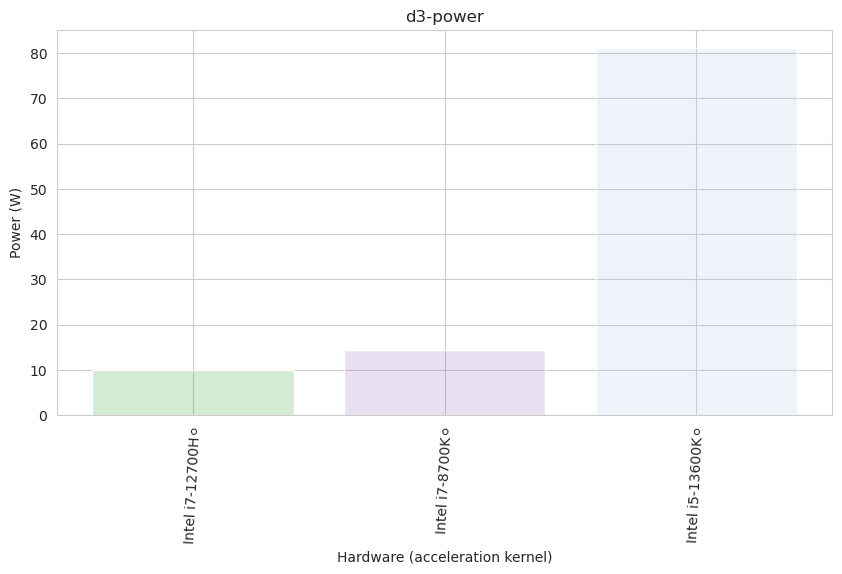}}
\caption{Best power results for \texttt{d3} benchmark.}
\label{subfig:a8blackboxgraph}
\end{subfigure}
\hfill % ensures that they are side by side

\caption{Best benchmark results for robot manipulation \texttt{d1}, \texttt{d2} and \texttt{d3}}
\label{fig:benchmarks_control_d1_d3}
\end{figure*}

\begin{figure*}[tbp]
\centering
    
% d4
\begin{subfigure}[t]{0.32\textwidth}  
\centering
\raisebox{-\height}{\includegraphics[width=\textwidth]{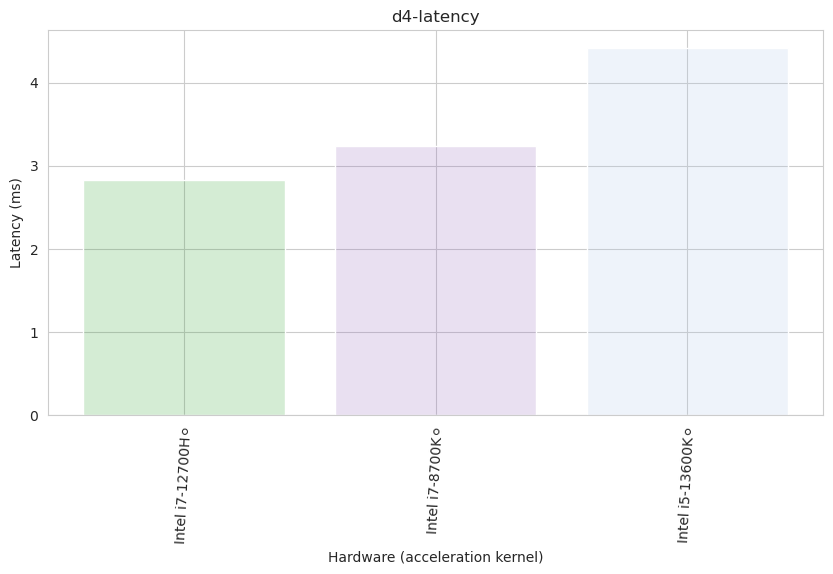}}
\caption{Best latency results for \texttt{d4} benchmark.}
\label{subfig:a8greyboxgraph}
\end{subfigure}
\hfill % ensures that they are side by side
\begin{subfigure}[t]{0.32\textwidth}
\centering
\raisebox{-\height}{\includegraphics[width=\textwidth]{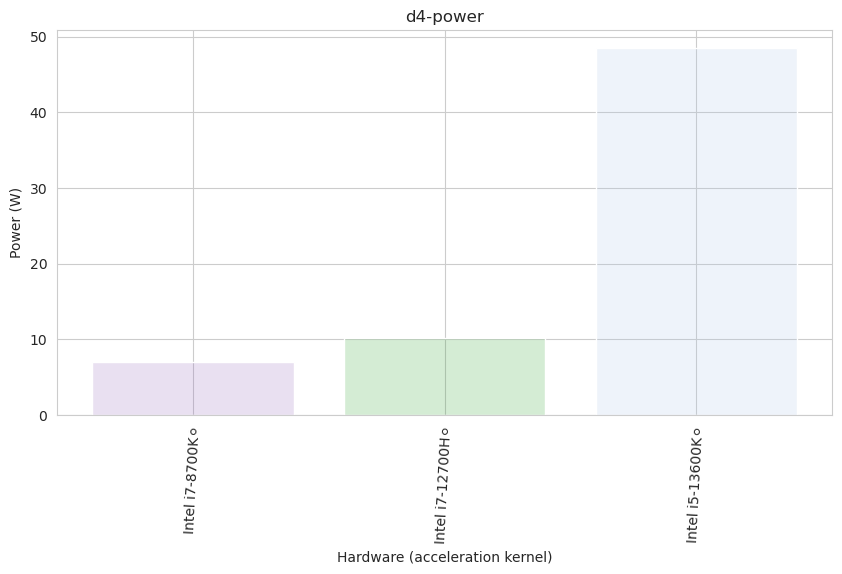}}
\caption{Best power results for \texttt{d4} benchmark.}
\label{subfig:a8blackboxgraph}
\end{subfigure}
\hfill % ensures that they are side by side
% d5
\begin{subfigure}[t]{0.32\textwidth}  
\centering
\raisebox{-\height}{\includegraphics[width=\textwidth]{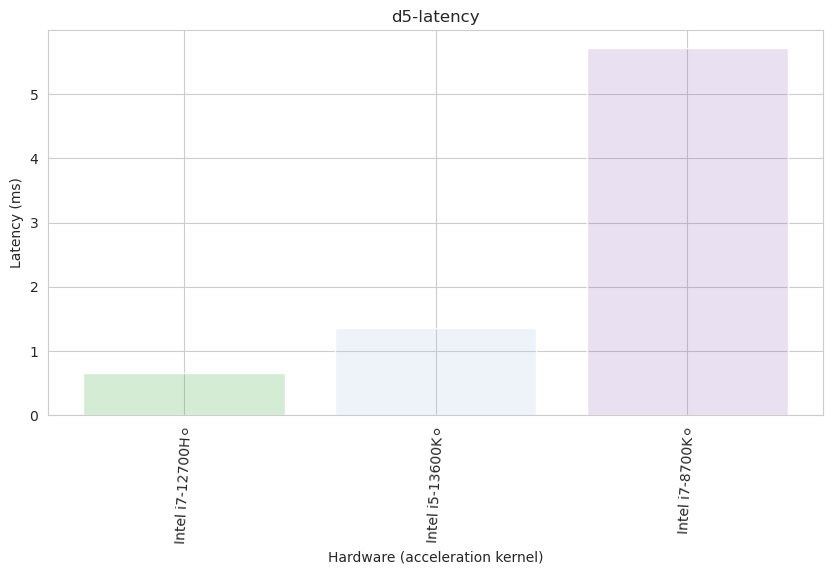}}
\caption{Best latency results for \texttt{d5} benchmark.}
\label{subfig:a8greyboxgraph}
\end{subfigure}
\hfill % ensures that they are side by side
\begin{subfigure}[t]{0.32\textwidth}
\centering
\raisebox{-\height}{\includegraphics[width=\textwidth]{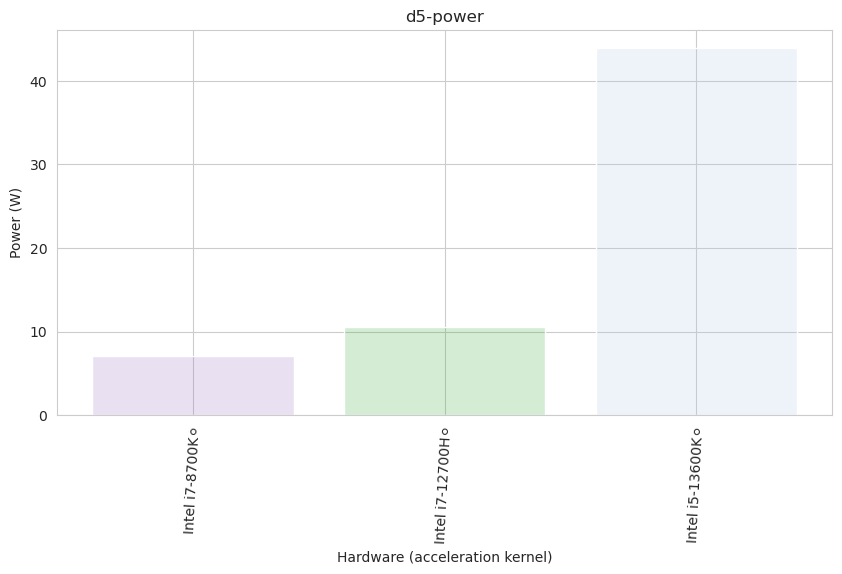}}
\caption{Best power results for \texttt{d5} benchmark.}
\label{subfig:a8blackboxgraph}
\end{subfigure}
\hfill % ensures that they are side by side
% d6
\begin{subfigure}[t]{0.32\textwidth}  
\centering
\raisebox{-\height}{\includegraphics[width=\textwidth]{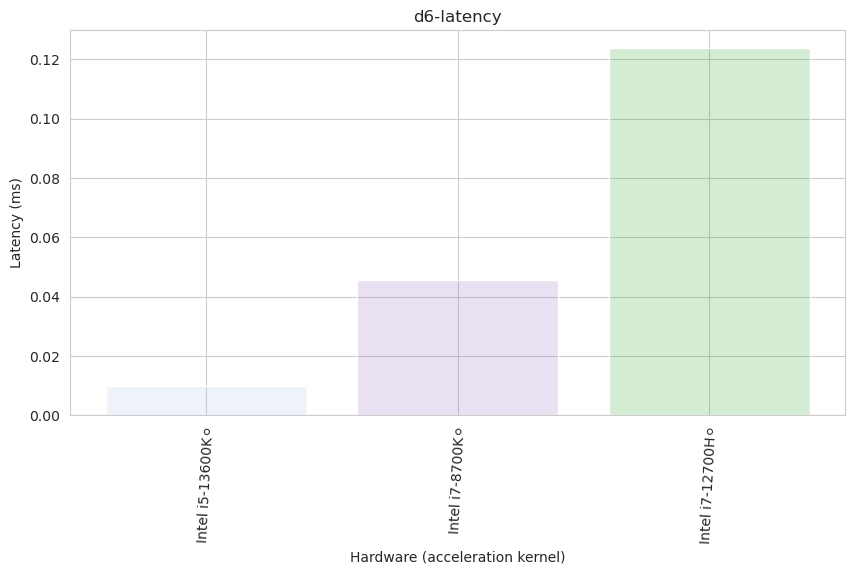}}
\caption{Best latency results for \texttt{d6} benchmark.}
\label{subfig:a8greyboxgraph}
\end{subfigure}
\hfill % ensures that they are side by side
\begin{subfigure}[t]{0.32\textwidth}
\centering
\raisebox{-\height}{\includegraphics[width=\textwidth]{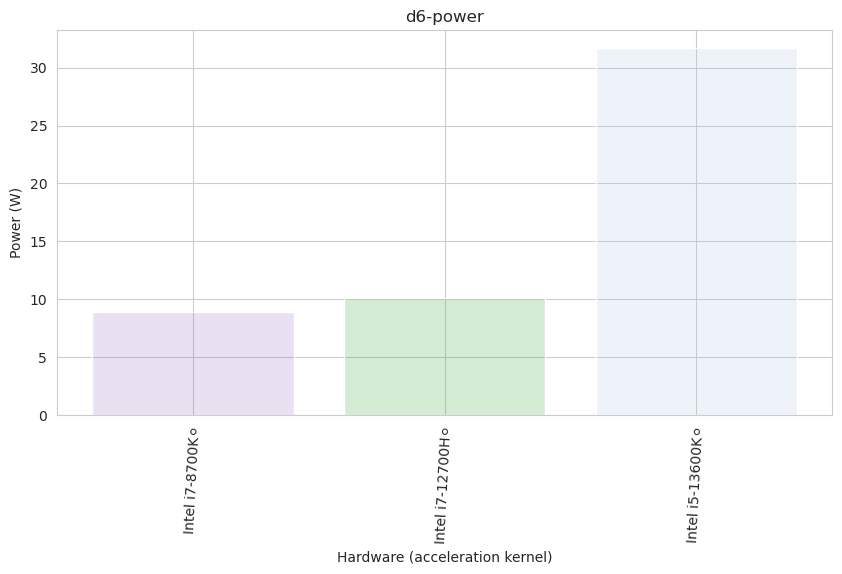}}
\caption{Best power results for \texttt{d6} benchmark.}
\label{subfig:a8blackboxgraph}
\end{subfigure}
\hfill % ensures that they are side by side
\caption{Best benchmark results for robot manipulation \texttt{d4}, \texttt{d5} and \texttt{d6}}
\label{fig:benchmarks_manipulation_d4_d6}
\end{figure*}

%%%%%%%%%%%%%%%%%%%%%%%%%%%%%%%%%%%%%%%%%%%%%%%%%%%%%%%%%%%%%%%%%

\label{sec:appendix_statistical_significance}

\begin{figure*}[tbp]
\centering

% a1-a3
\begin{subfigure}[t]{0.32\textwidth}  
\centering
\raisebox{-\height}{\includegraphics[width=\textwidth]{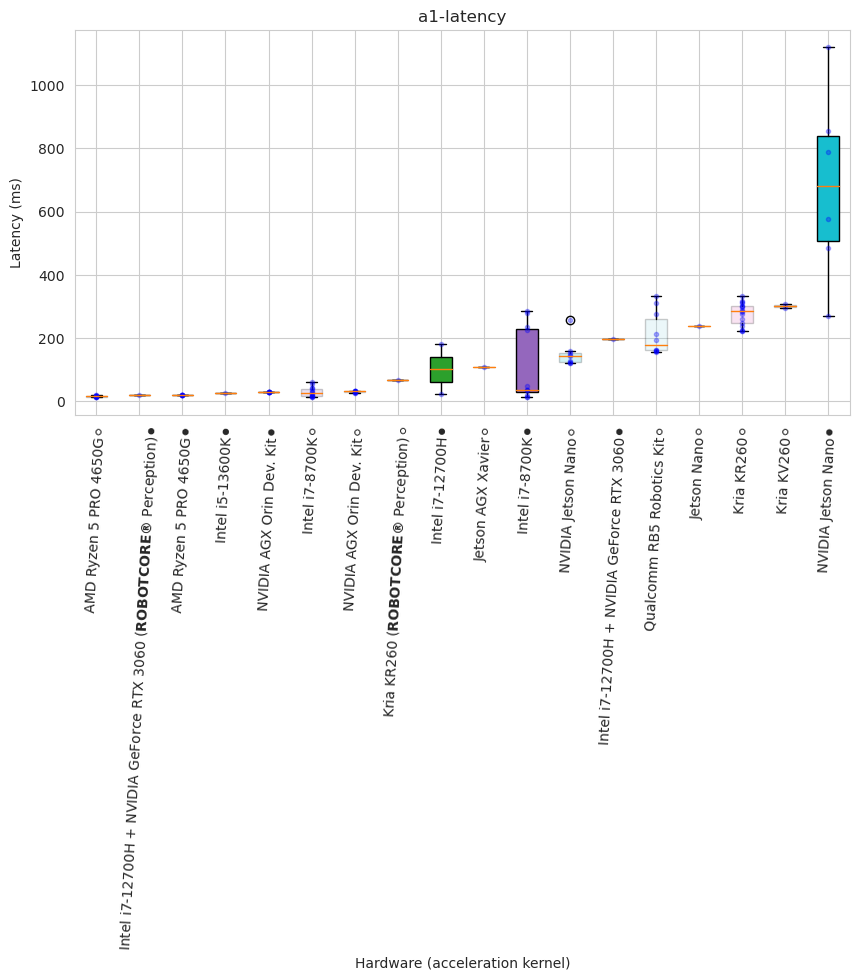}}
\caption{Latency results for \texttt{a1} benchmark with statistical significance.}
\label{subfig:latstatisticsa1}
\end{subfigure}
\hfill % ensures that they are side by side
\begin{subfigure}[t]{0.32\textwidth}
\centering
\raisebox{-\height}{\includegraphics[width=\textwidth]{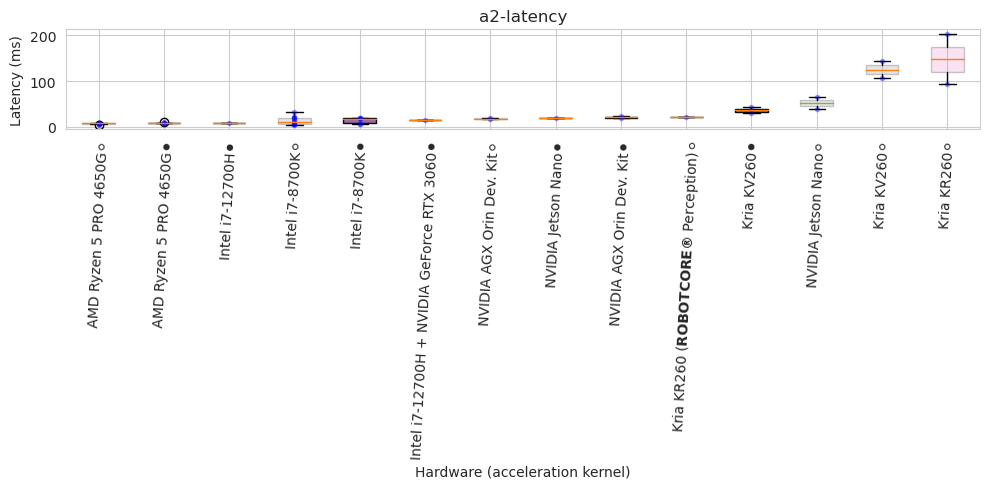}}
\caption{Latency results for \texttt{a2} benchmark with statistical significance.}
\label{subfig:latstatisticsa2}
\end{subfigure}
\hfill % ensures that they are side by side
\begin{subfigure}[t]{0.32\textwidth}
\centering
\raisebox{-\height}{\includegraphics[width=\textwidth]{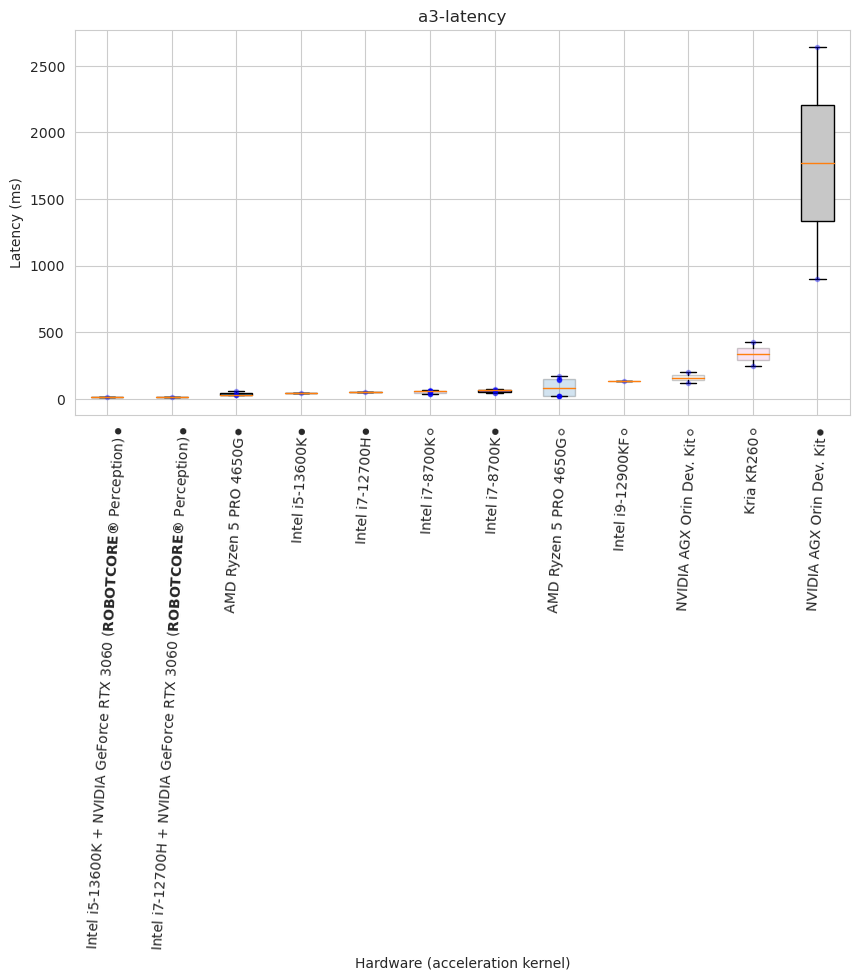}}
\caption{Latency results for \texttt{a3} benchmark  with statistical significance.}
\label{subfig:latstatisticsa3}
\end{subfigure}

\hfill

% a4-b1
\begin{subfigure}[t]{0.32\textwidth}  
\centering
\raisebox{-\height}{\includegraphics[width=\textwidth]{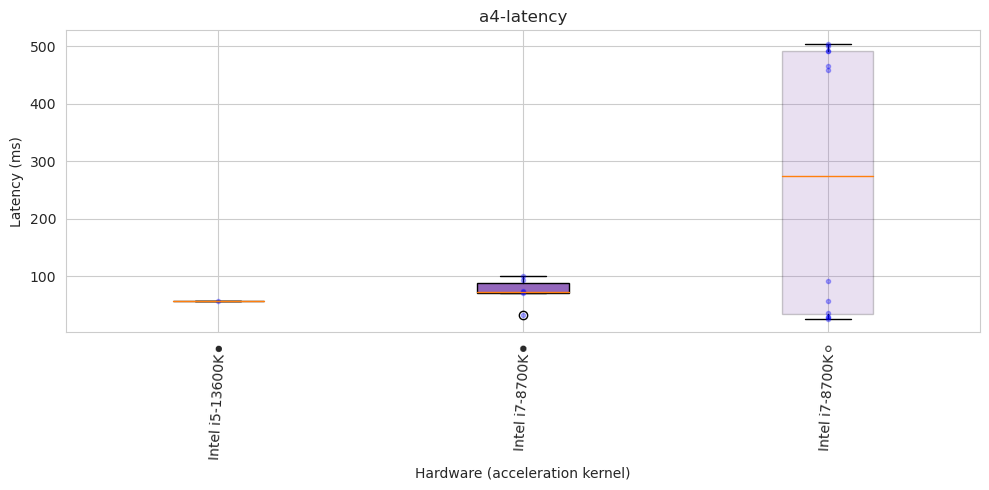}}
\caption{Latency results for \texttt{a5} benchmark with statistical significance.}
\label{subfig:latstatisticsa4}
\end{subfigure}
\hfill % ensures that they are side by side
\begin{subfigure}[t]{0.32\textwidth}
\centering
\raisebox{-\height}{\includegraphics[width=\textwidth]{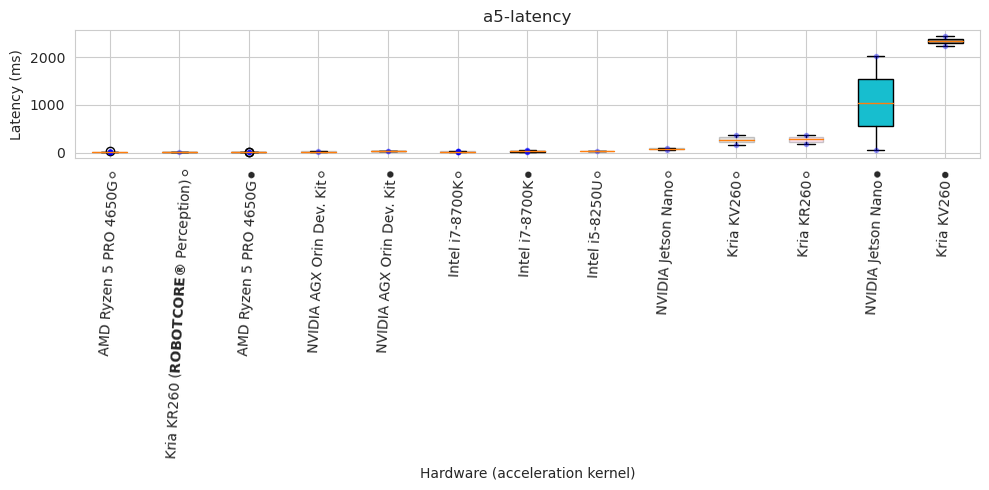}}
\caption{Latency results for \texttt{a5} benchmark with statistical significance.}
\label{subfig:latstatisticsa5}
\end{subfigure}
\hfill % ensures that they are side by side
\begin{subfigure}[t]{0.32\textwidth}
\centering
\raisebox{-\height}{\includegraphics[width=\textwidth]{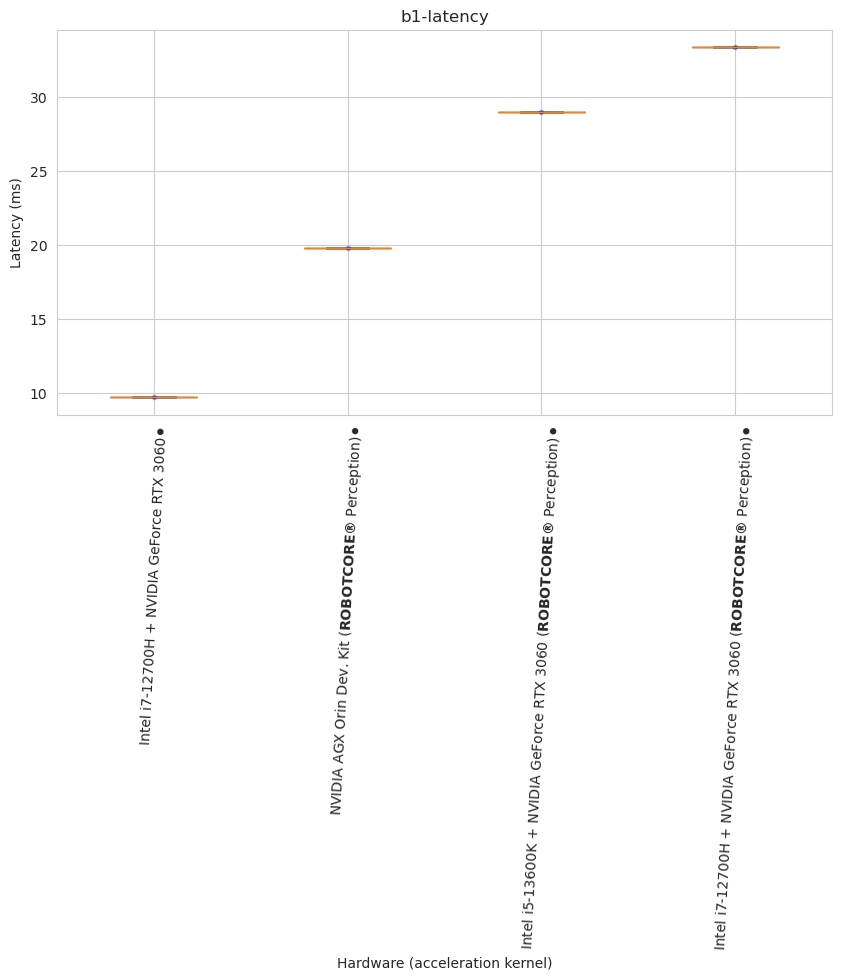}}
\caption{Latency results for \texttt{b1} benchmark  with statistical significance.}
\label{subfig:latstatisticsb1}
\end{subfigure}

% b2-c1
\begin{subfigure}[t]{0.32\textwidth}  
\centering
\raisebox{-\height}{\includegraphics[width=\textwidth]{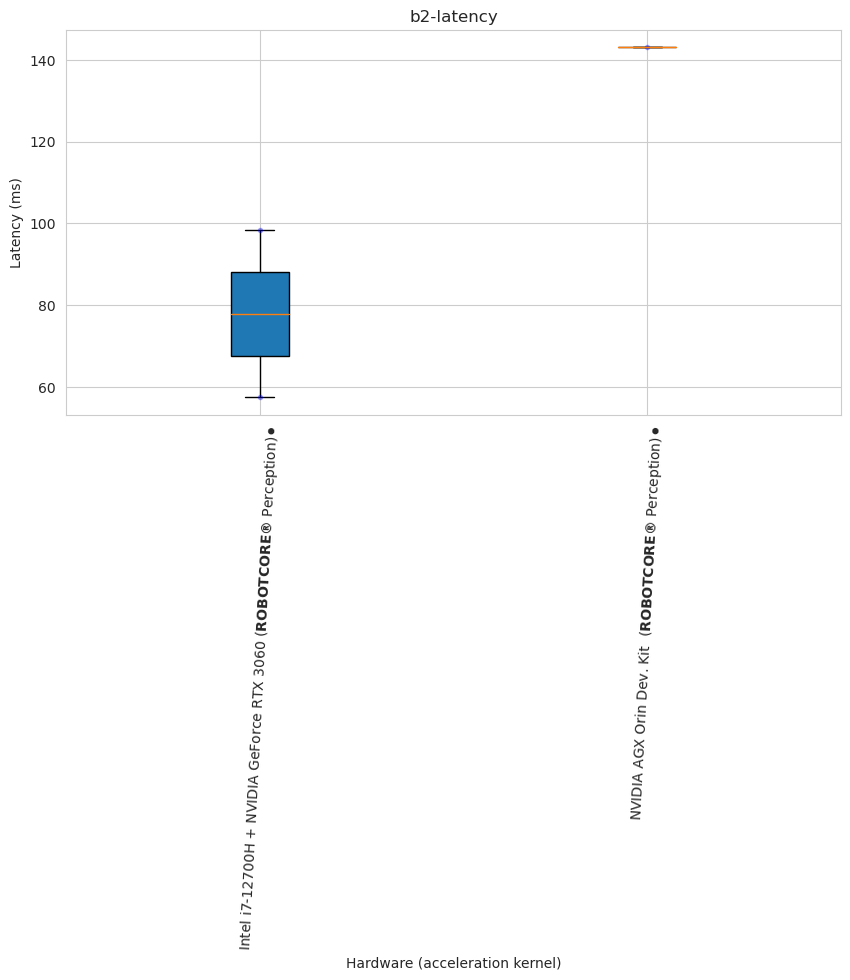}}
\caption{Latency results for \texttt{b2} benchmark with statistical significance.}
\label{subfig:latstatisticsb2}
\end{subfigure}
\hfill % ensures that they are side by side
\begin{subfigure}[t]{0.32\textwidth}
\centering
\raisebox{-\height}{\includegraphics[width=\textwidth]{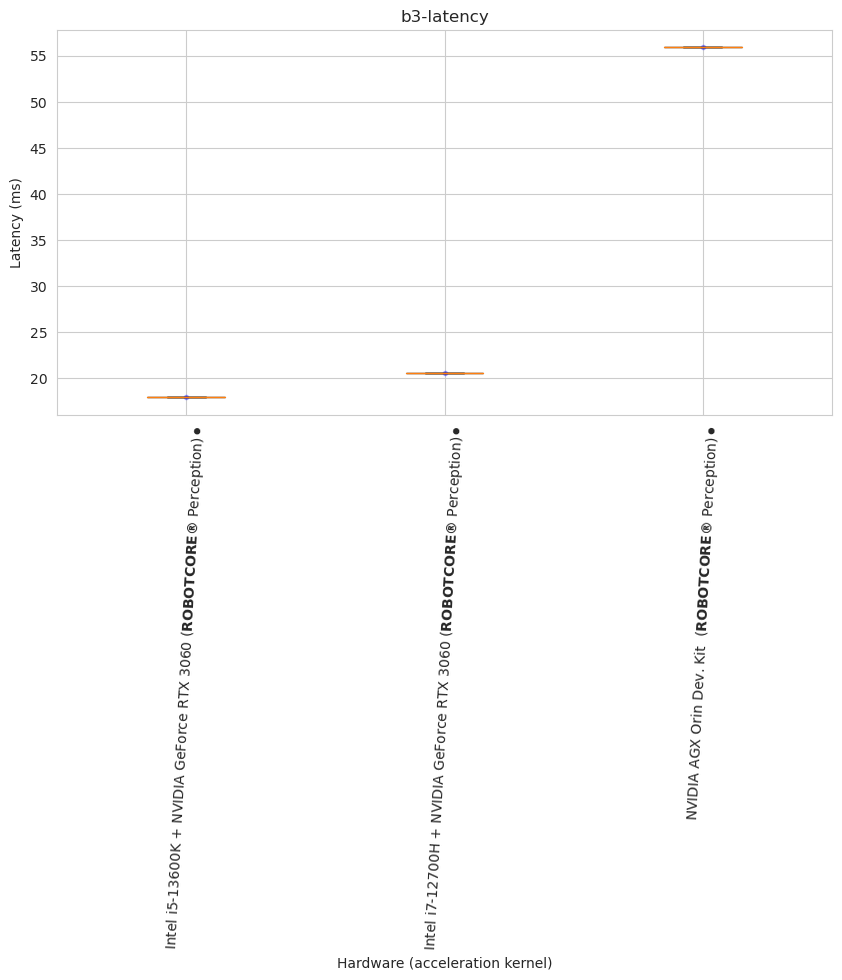}}
\caption{Latency results for \texttt{b3} benchmark with statistical significance.}
\label{subfig:latstatisticsb3}
\end{subfigure}
\hfill % ensures that they are side by side
\begin{subfigure}[t]{0.32\textwidth}
\centering
\raisebox{-\height}{\includegraphics[width=\textwidth]{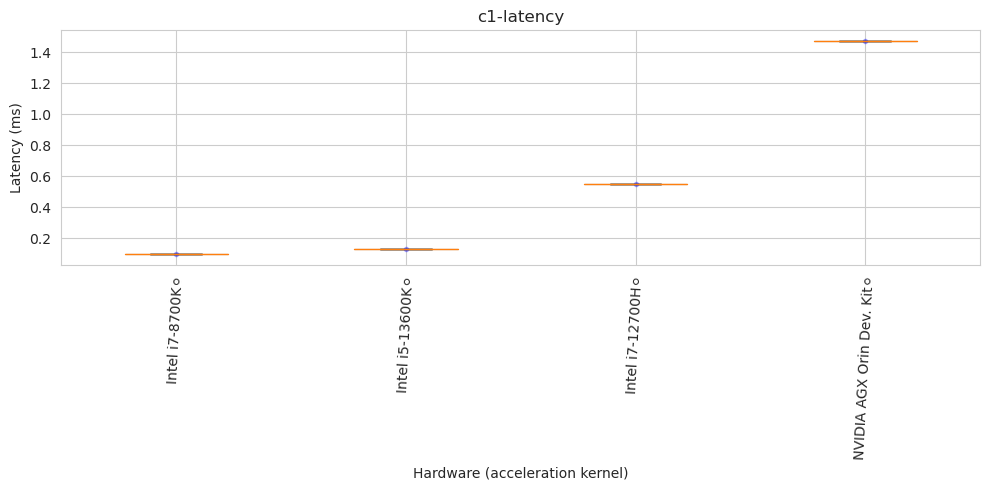}}
\caption{Latency results for \texttt{c1} benchmark  with statistical significance.}
\label{subfig:latstatisticsc1}
\end{subfigure}

\caption{Benchmarks \texttt{a1} to \texttt{c1} with additional statistical significance.}
\label{fig:benchmarks_statistics_a1_c1}
\end{figure*}

\begin{figure*}[tbp]
\centering

% c2-c4
\begin{subfigure}[t]{0.32\textwidth}  
\centering
\raisebox{-\height}{\includegraphics[width=\textwidth]{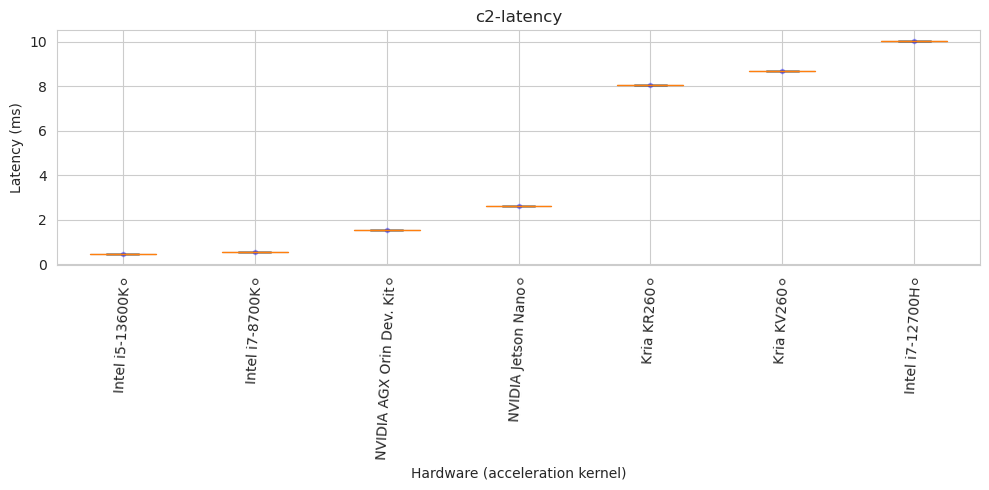}}
\caption{Latency results for \texttt{c2} benchmark with statistical significance.}
\label{subfig:latstatisticsc2}
\end{subfigure}
\hfill % ensures that they are side by side
\begin{subfigure}[t]{0.32\textwidth}
\centering
\raisebox{-\height}{\includegraphics[width=\textwidth]{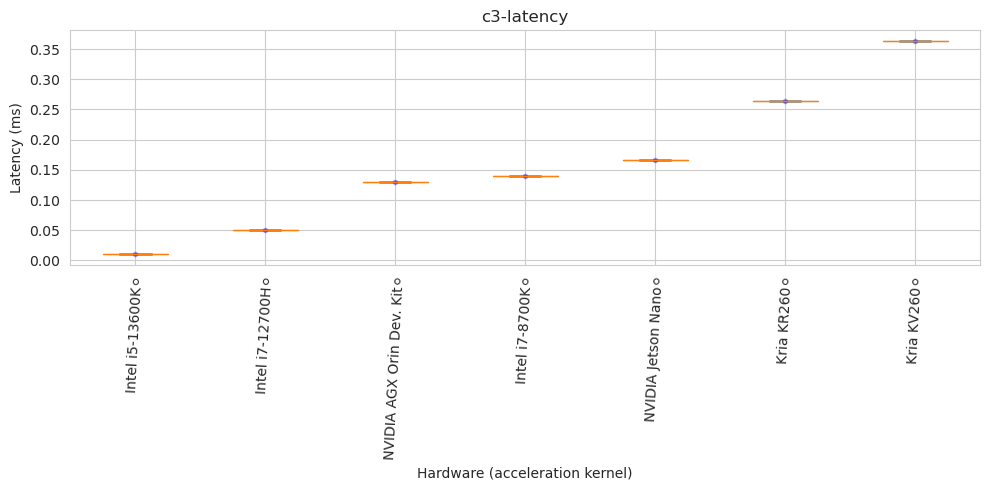}}
\caption{Latency results for \texttt{c3} benchmark with statistical significance.}
\label{subfig:latstatisticsc3}
\end{subfigure}
\hfill % ensures that they are side by side
\begin{subfigure}[t]{0.32\textwidth}
\centering
\raisebox{-\height}{\includegraphics[width=\textwidth]{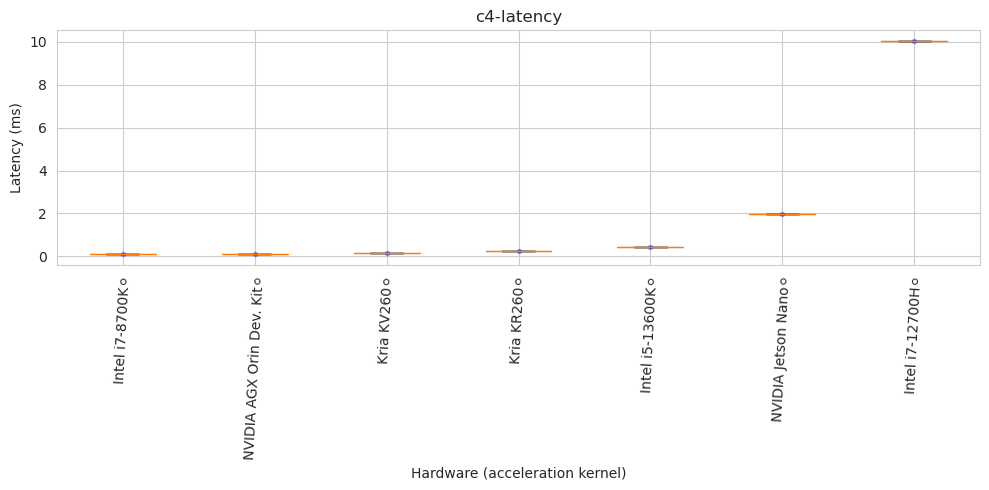}}
\caption{Latency results for \texttt{c4} benchmark  with statistical significance.}
\label{subfig:latstatisticsc4}
\end{subfigure}

\hfill

% c5-d2
\begin{subfigure}[t]{0.32\textwidth}  
\centering
\raisebox{-\height}{\includegraphics[width=\textwidth]{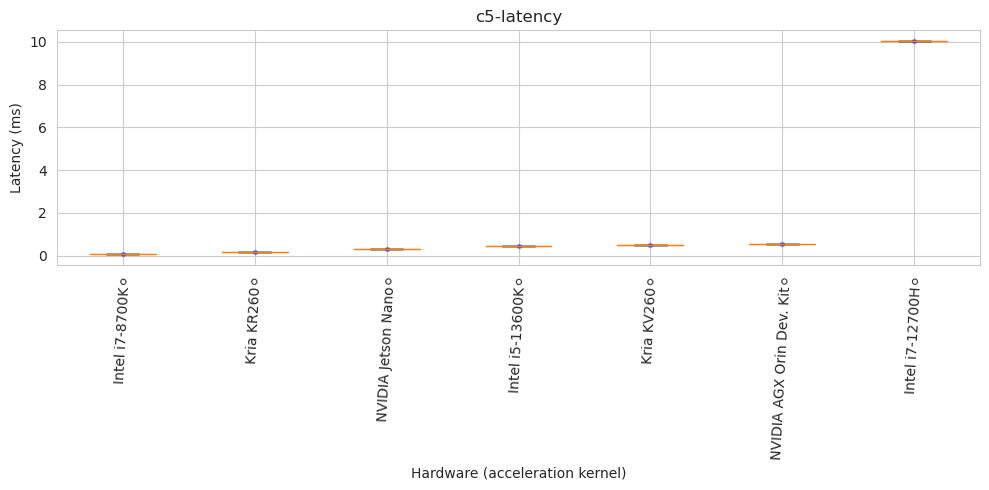}}
\caption{Latency results for \texttt{c5} benchmark with statistical significance.}
\label{subfig:latstatisticsc5}
\end{subfigure}
\hfill % ensures that they are side by side
\begin{subfigure}[t]{0.32\textwidth}
\centering
\raisebox{-\height}{\includegraphics[width=\textwidth]{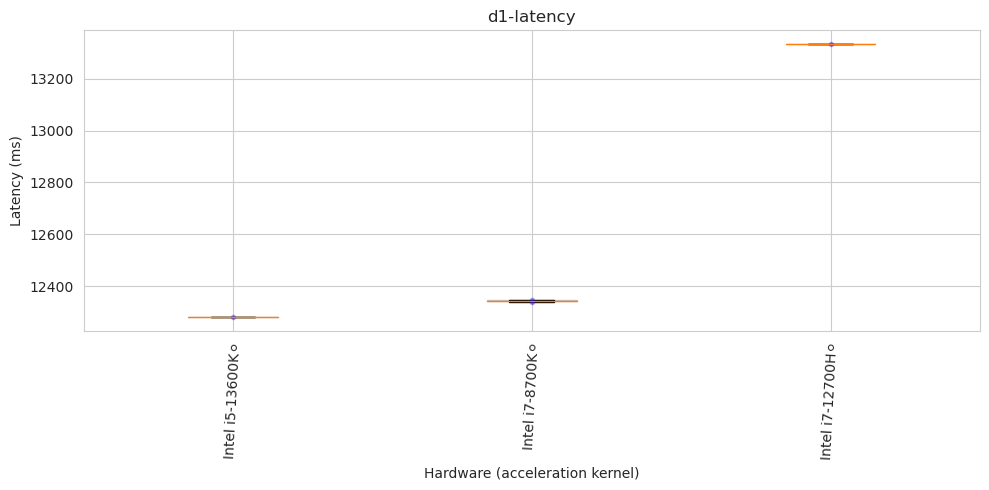}}
\caption{Latency results for \texttt{d1} benchmark with statistical significance.}
\label{subfig:latstatisticsd1}
\end{subfigure}
\hfill % ensures that they are side by side
\begin{subfigure}[t]{0.32\textwidth}
\centering
\raisebox{-\height}{\includegraphics[width=\textwidth]{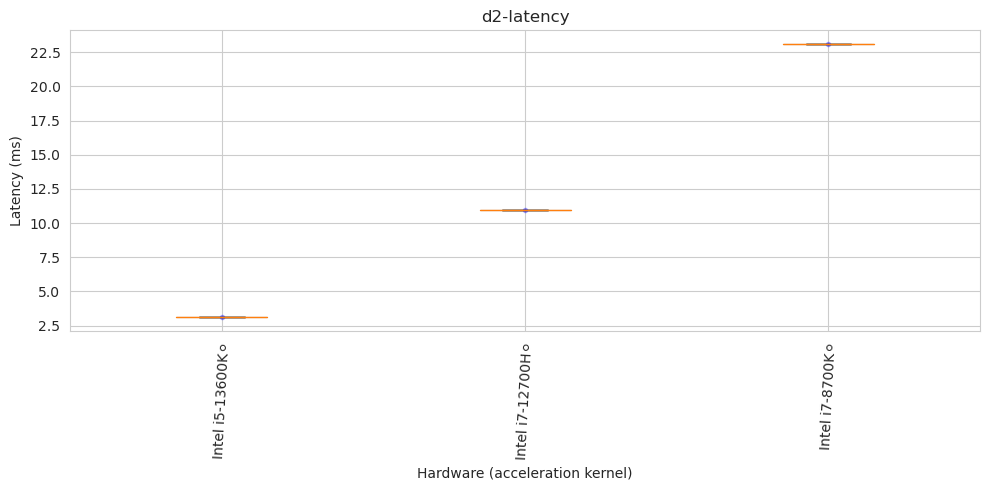}}
\caption{Latency results for \texttt{d2} benchmark  with statistical significance.}
\label{subfig:latstatisticsd2}
\end{subfigure}

% d3-d5
\begin{subfigure}[t]{0.32\textwidth}  
\centering
\raisebox{-\height}{\includegraphics[width=\textwidth]{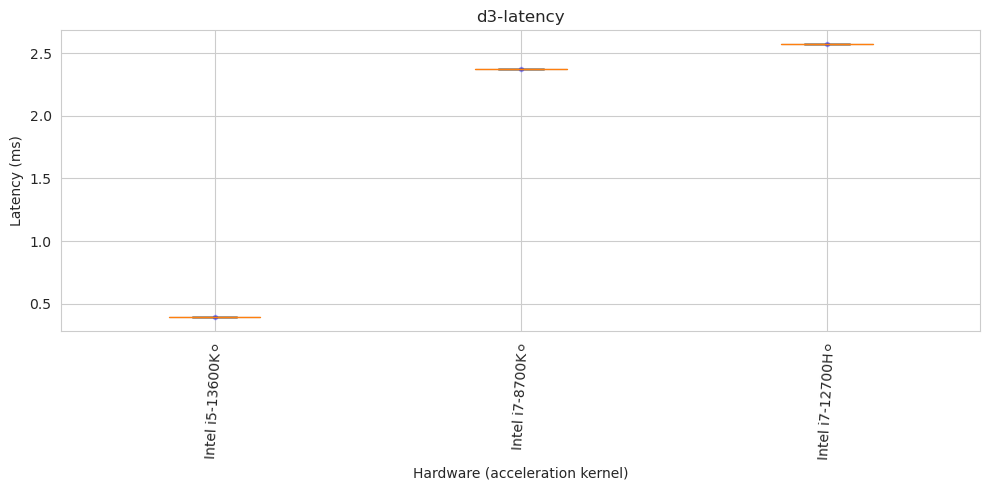}}
\caption{Latency results for \texttt{d3} benchmark with statistical significance.}
\label{subfig:latstatisticsd3}
\end{subfigure}
\hfill % ensures that they are side by side
\begin{subfigure}[t]{0.32\textwidth}
\centering
\raisebox{-\height}{\includegraphics[width=\textwidth]{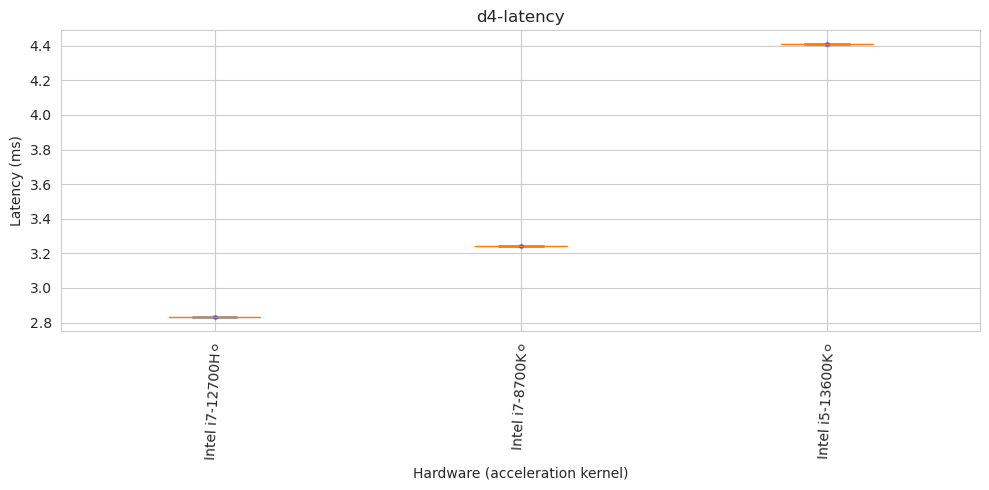}}
\caption{Latency results for \texttt{d4} benchmark with statistical significance.}
\label{subfig:latstatisticsd4}
\end{subfigure}
\hfill % ensures that they are side by side
\begin{subfigure}[t]{0.32\textwidth}
\centering
\raisebox{-\height}{\includegraphics[width=\textwidth]{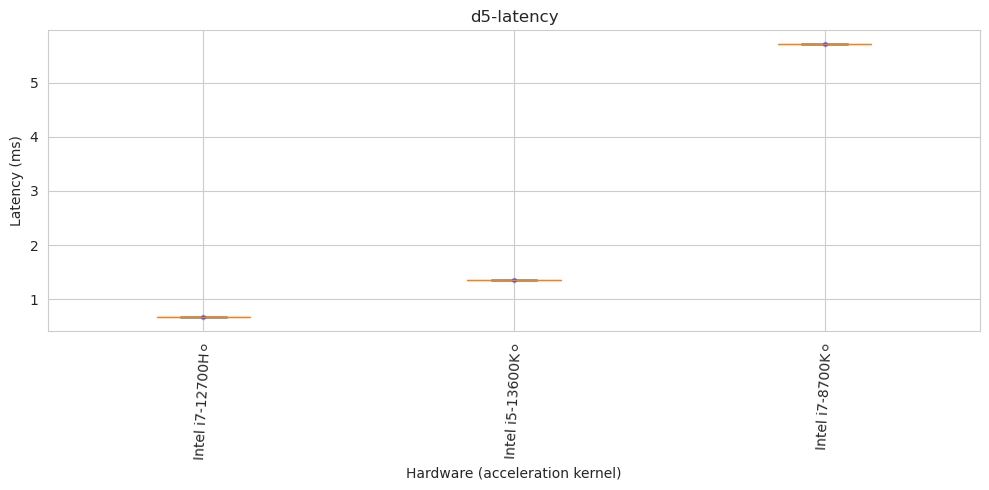}}
\caption{Latency results for \texttt{d5} benchmark  with statistical significance.}
\label{subfig:latstatisticsd5}
\end{subfigure}

\caption{Benchmarks \texttt{c2} to \texttt{d5} with additional statistical significance.}
\label{fig:benchmarks_statistics_c2_d5}
\end{figure*}
